# Supplementary material for: First Measurement of Energy-Dependent Inclusive Muon Neutrino Charged-Current Cross Sections on Argon with the MicroBooNE Detector
Source: arXiv:2110.14023 ancillary file (2022-04-12)
Supplement: Supplementary file 1 [file Supplemental.pdf]

# Supplemental Materials for: "First Measurement of Energy-dependent Inclusive Muon Neutrino Charged-Current Cross Sections on Argon with the MicroBooNE Detector"

MicroBooNE Collaboration

## I. PERFORMANCE OF INCLUSIVE $\nu_\mu$ CC EVENT SELECTION

Fig. 1 and Fig. 2 show the comparison between data and Monte Carlo (MC) predictions for fully-contained (FC) and partially contained (PC) events, respectively, as a function of reconstructed neutrino energy, reconstructed muon energy, reconstructed cosine of muon polar angle relative to the neutrino beam direction, and reconstructed hadronic energy. Within each plot, we include the goodness-of-fit test[1] ($\chi^2/ndf$ with ndf being the number of bins) for each measurement as well as the total normalization ratio. For Monte Carlo simulation, we further break down the selection results into different interaction types using the truth information. From these plots, all major interaction types (CCQE: charged-current quasi-elastic scattering, CCMEC: charged-current meson-exchange-current interaction, CCRES: charged-current resonance production, CCDIS: charged-current deep-inelastic-scattering scattering, etc.) have been selected without obvious efficiency holes. The efficiencies for each interaction type are plotted as a function of true neutrino energy, true muon energy, true cosine of muon polar angle relative to the neutrino beam direction, and true energy transfer in Fig. 3, Fig. 4, Fig. 5, and Fig. 6, respectively.

While the efficiencies are generally different for different interaction types, they are quite consistent to each other as a function of the cosine muon polar angle ($\cos\theta$) relative to the beam direction. This behaviour is consistent with the expectation given that the muon polar angle is a key kinematic variable for distinguishing signals from background (cosmic-ray muons or neutral current interactions). Thus we are confident that this $\nu_\mu$CC event selection is largely inclusive with respect to different interaction types. For CCMEC, the reduction of efficiency at the backward angle may be attributed to the events with invisible protons in the final states, in which case a single backward-going muon will be more likely attributed tagged as cosmic-rays. The efficiencies in other kinematic spaces depend on their event distributions as well as the underlying muon angle distribution in each bin. For example, in neutrino or muon energy space, the CCMEC and CCothers (mostly CC-COH: charged-current coherent scattering) in general have relatively higher efficiencies than other interaction types because their muon angle distributions are more forward-going.

## II. VALIDATION OF OVERALL MODEL

The (differential) cross-section extraction with the Wiener-SVD unfolding method is essentially a linear transformation (or re-smearing) of the measured event distribution. To ensure the uncertainties of the unfolded cross sections have proper coverage, it is important to demonstrate the measured event distribution is consistent with the overall model within its uncertainties. In the following, we summarize these validations. In particular, as shown in Sec. II E, we performed the conditional goodness-of-fit (GoF) test on the hadronic energy $E_{had}$ after applying the constraints to the muon kinematics for selected $\nu_\mu$CC candidates. This test can be used to directly validate the modeling of missing energy (e.g. neutrons or low-energy photons) in the neutrino-argon interaction.

### A. Construction of test statistics

We adopted the covariance matrix formalism to construct the $\chi^2$ test statistic:

$$\chi^2 = (M-P)^T \times Cov^{-1}_{full}(M,P) \times (M-P), \quad (1)$$

where $M$ and $P$ are vectors of measurement and prediction, respectively. Here, the prediction includes the contributions from both signal and background. The $Cov(M,P)$ is the full covariance matrix:

$$Cov = Cov^{stat}_{Pearson} + Cov^{stat}_{MC} + Cov^{sys}_{xs} + Cov^{sys}_{flux} + Cov^{sys}_{det} + Cov^{sys}_{add}, \quad (2)$$

[1] See detailed definition in Eq. 1. The interpretation of $\chi^2/ndf$ value should be done in p-value, which can be calculated based on the reported $\chi^2/ndf$ and is considered to be acceptable if the p-value is larger than 0.05.

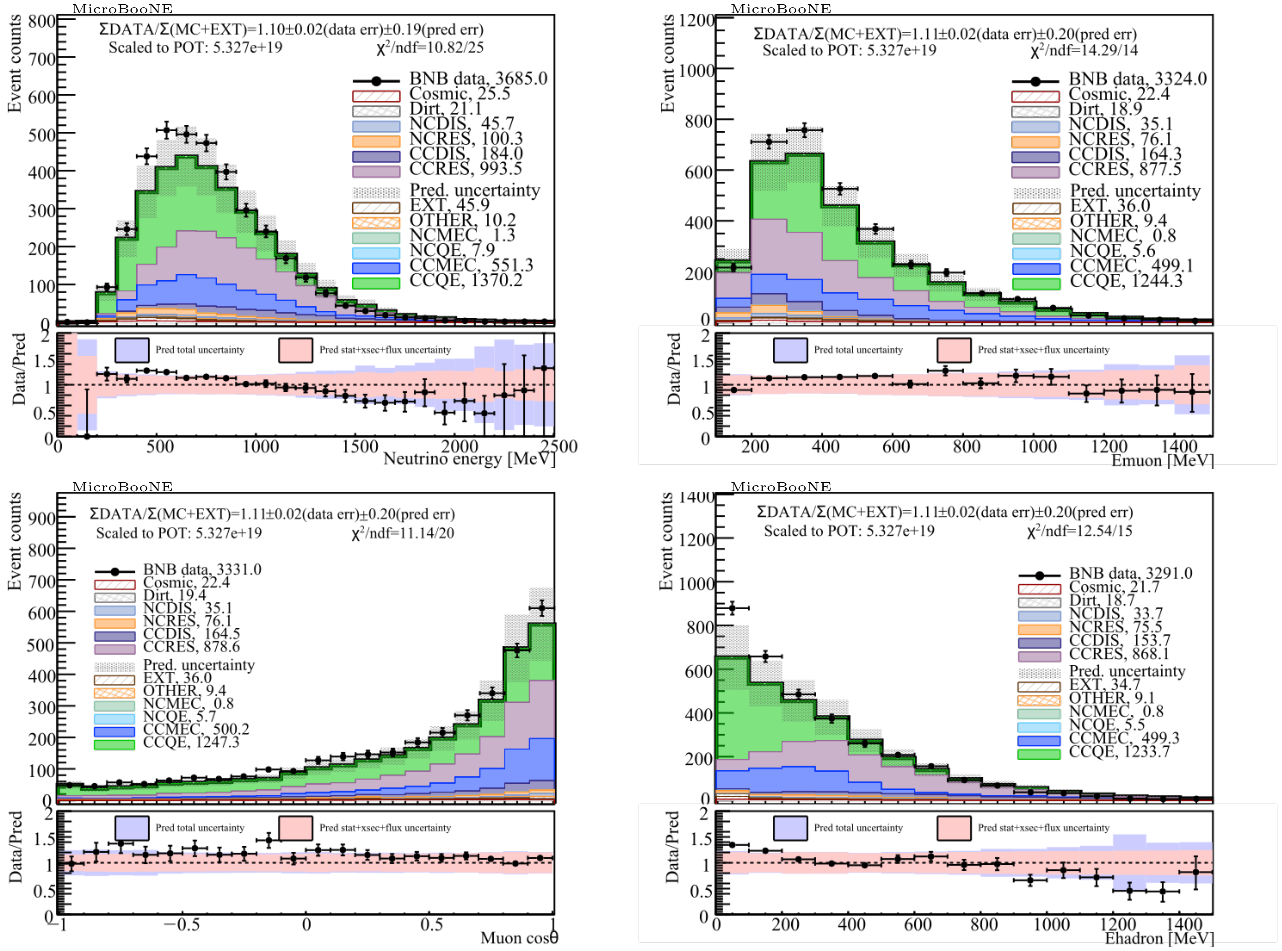


FIG. 1. The $\nu_\mu$CC selections, from $5.3{\times}10^{19}$ POT data, for fully-contained (FC) events, with a breakdown into different interaction types. The stippled band on the top panel of each sub-figure represents the total systematic uncertainties. The data/MC ratio is plotted in the bottom panel. The pink uncertainty band includes only the neutrino flux, cross section and MC statistical uncertainties. The purple uncertainty band additionally includes uncertainties in the detector modeling.

where $Cov^{stat}_{Pearson}$ is a covariance matrix constructed based on the Pearson method [1, 2] with the diagonal terms filled with the square of the statistical uncertainty of prediction in the $i$th bin. The $Cov^{stat}_{MC}$ is the diagonal covariance matrix containing the statistical uncertainties corresponding to finite statistics from Monte Carlo simulations. The other four covariance matrices $Cov^{sys}_{xs}$, $Cov^{sys}_{flux}$, $Cov^{sys}_{det}$, $Cov^{sys}_{add}$, are the covariance matrices corresponding to uncertainties from cross section, neutrino flux, detector performance, and additional uncertainties from the "dirt" contribution, respectively.

### B. Goodness-of-fit calculation

With the $\chi^2$ test statistic defined above, we can perform the goodness-of-fit (GoF) test. Given the null hypothesis (i.e. the overall model), the $\chi^2$ value can be used to perform the GoF test by comparing with the $\chi^2$ distribution with the corresponding number of degrees of freedom. The above GoF test provides an overall evaluation of the model with the data. This evaluation can be zoomed into different parts of the model using the conditional covariance matrix formalism [3]. For example, given the full covariance (stat. + syst.) containing two channels (X, Y):

$$\Sigma = \begin{pmatrix} \Sigma^{XX} & \Sigma^{XY} \\ \Sigma^{YX} & \Sigma^{YY} \end{pmatrix}, \quad n: \text{measurement}, \quad \mu: \ \text{prediction}, \tag{3}$$

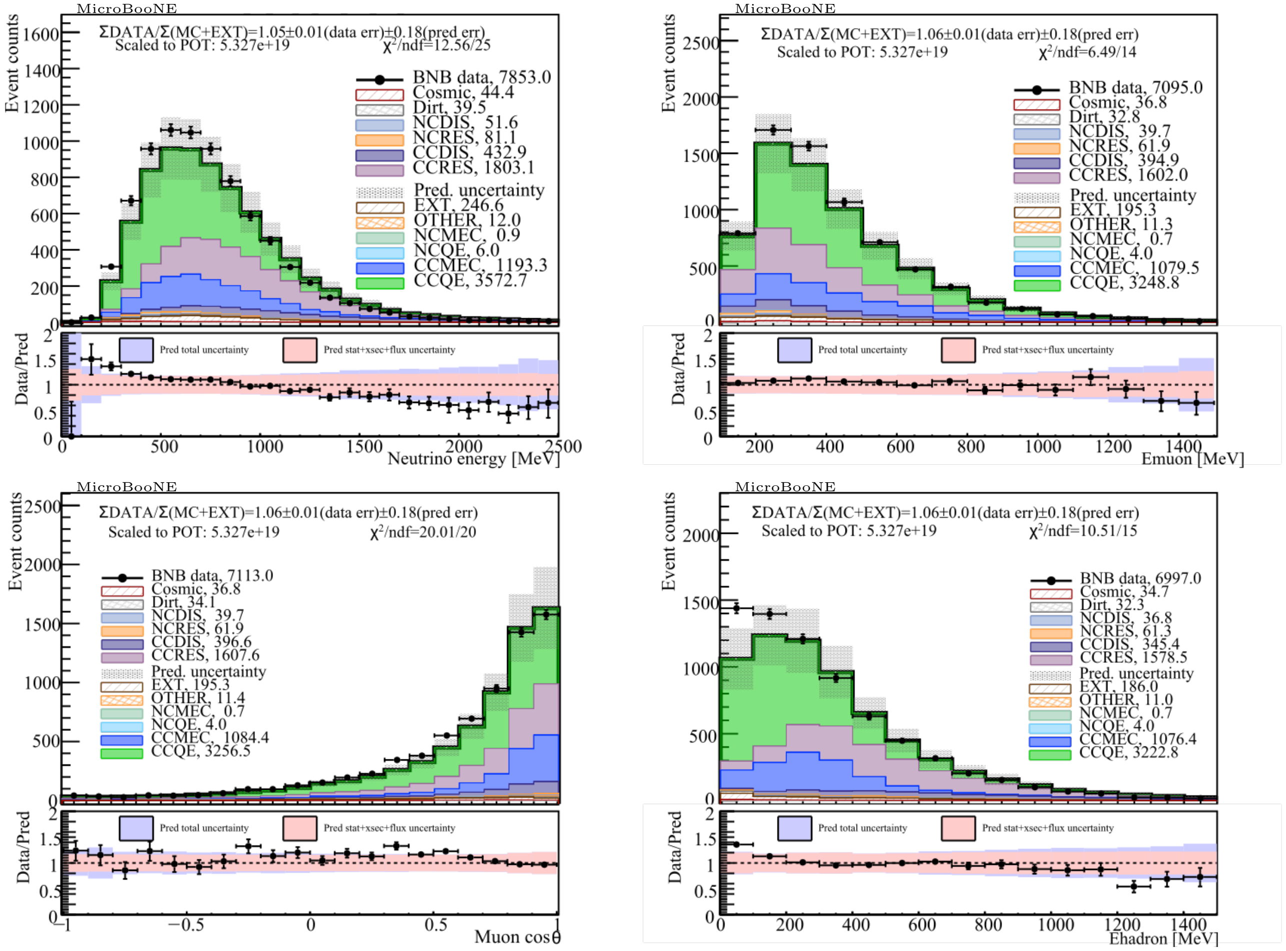


FIG. 2. Similar as Fig. 1 but for partially contained (PC) events.

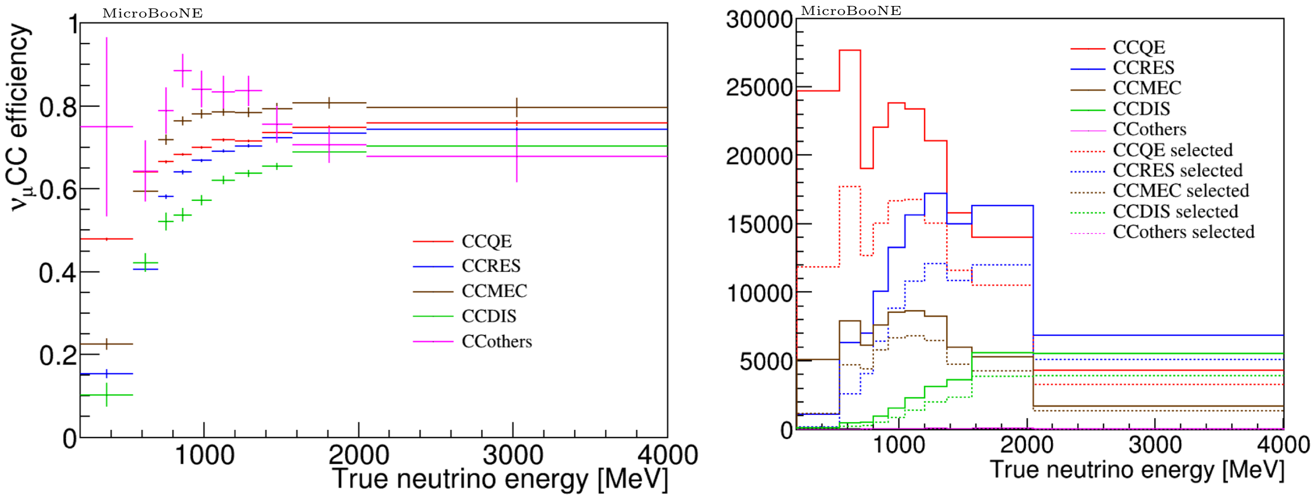


FIG. 3. (Left) Efficiencies of $\nu_\mu$CC selection as a function of true neutrino energy for different interaction types. (Right) Event distributions before and after selection. The binning is chosen to be the same as the unfolded total cross section. The error bar includes statistical uncertainty.

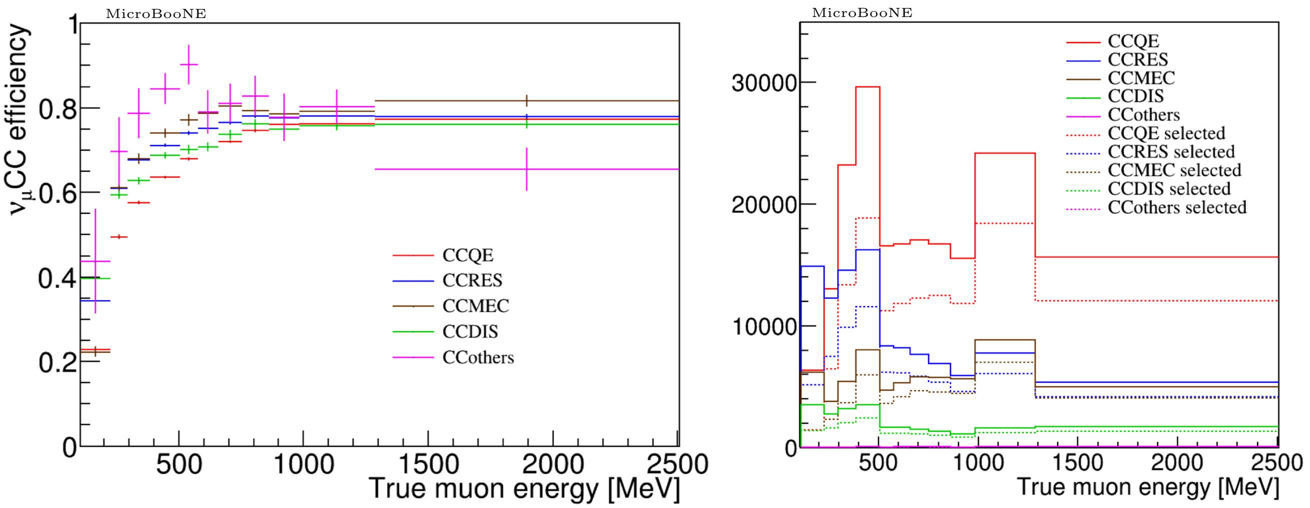


FIG. 4. (Left) Efficiencies of $\nu_\mu$CC selection as a function of true muon energy for different interaction types. (Right) Event distributions before and after selection. The binning is chosen to be the same as the unfolded differential cross section. The error bar includes statistical uncertainty.

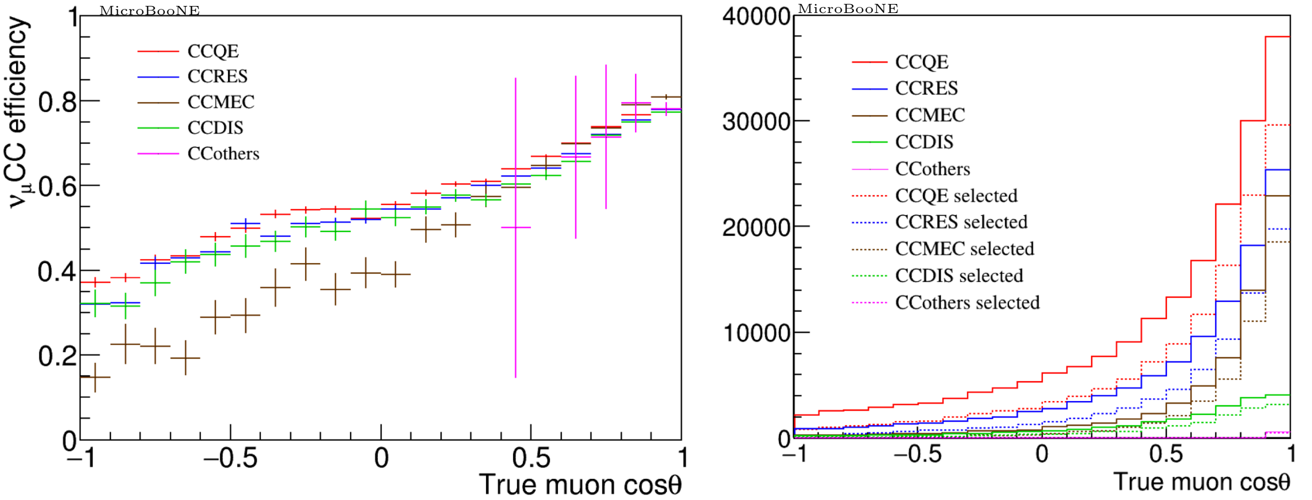


FIG. 5. (Left) Efficiencies of $\nu_\mu$CC selection as a function of true muon cos$\theta$ for different interaction types. (Right) Event distributions before and after selection. The error bar includes statistical uncertainty.

we can derive the prediction on $X$ given the constraints on $Y$:

$$\mu^{X,constrained} = \mu^X + \Sigma^{XY} \times \left(\Sigma^{YY}\right)^{-1} \times \left(n^Y - \mu^Y\right), \quad (4)$$

$$\Sigma^{XX,constrained} = \Sigma^{XX} - \Sigma^{XY} \times \left(\Sigma^{YY}\right)^{-1} \times \Sigma^{YX}. \quad (5)$$

Thus, a GoF test can be performed on $Y$ first, and then performed on $X$ after the constraints of $Y$. This allows the examination of the model on $X$ and $Y$ individually. For example, we can examine the GoF of PC $\nu_\mu$CC given the constraints to the measured FC $\nu_\mu$CC distribution.

### C. GoF Tests of various $\nu_\mu$CC Distributions

In the following three sections, we present the goodness-of-fit (GoF) of various $\nu_\mu$CC distributions from BNB data corresponding to $5.327\times10^{19}$ protons-on-target (POT). We also show the GoFs without considering the detector systematics, which allows for more stringent tests on the overall model. Figure 7 shows the comparison between data and

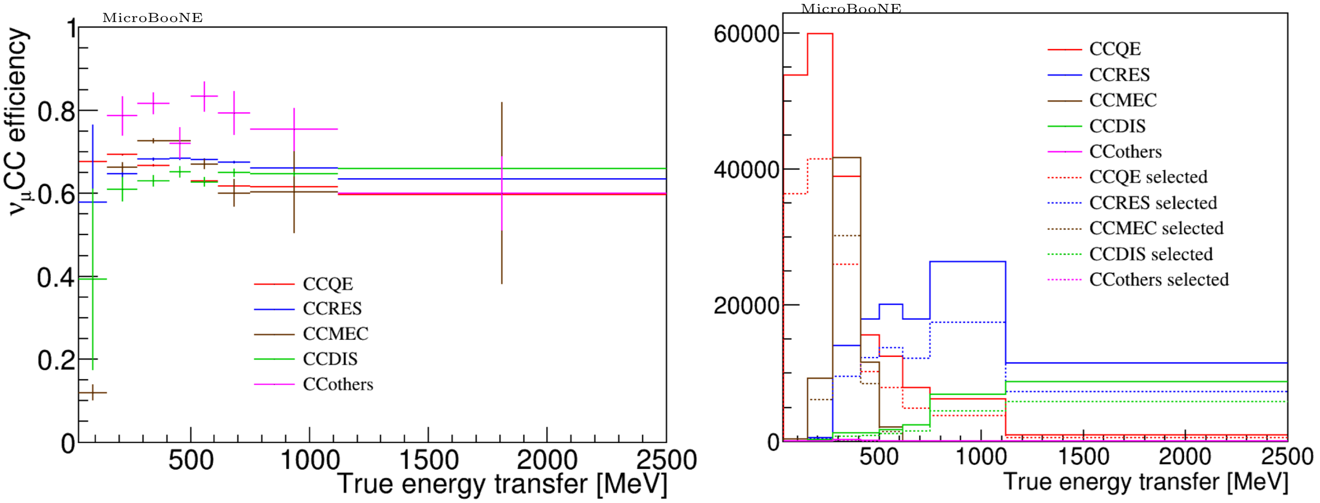


FIG. 6. (Left) Efficiencies of $\nu_\mu$CC selection as a function of true energy transfer for different interaction types. (Right) Event distributions before and after selection. The binning is chosen to be the same as the unfolded differential cross section. The error bar includes statistical uncertainty.

prediction as a function of the reconstructed muon energy $E_\mu^{rec}$ for both fully contained (FC) and partially contained (PC) channels. Left (right) panel is shown with fully systematic uncertainties (without detector systematics). Even in the case without considering the detector systematics, the corresponding p-value of 0.54 ($\chi^2/ndf$=28.65/30) is still acceptable, showing good agreement between data and model prediction.

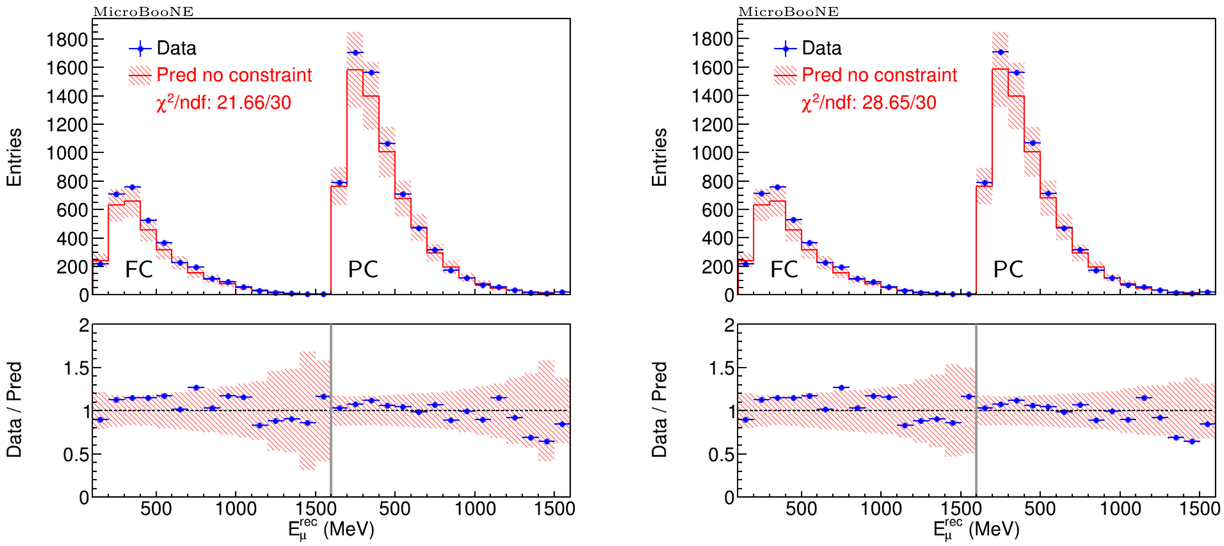


FIG. 7. Comparison between data and prediction as a function of $E_\mu^{rec}$: (left) all systematic uncertainties, (right) without detector systematic uncertainties. The statistical uncertainties of the data and Monte Carlo are also included in the bands. For each plot, the first 14 bins with 100 MeV per bin correspond to the fully contained events from 0.1 GeV to 1.5 GeV. The 15th bin is the overflow bin corresponding to fully contained events above 1.5 GeV. The next 14 bins with 100 MeV per bin correspond to the partially contained events from 0.1 GeV to 1.5 GeV. The last bin is the overflow bin corresponding to the partially contained events above 1.5 GeV.

Figure 8 shows the comparison between data and prediction as a function of the reconstructed cosine muon polar angle $\cos\theta_\mu^{rec}$ relative to the neutrino beam direction. Left (right) panel is shown with fully systematic uncertainties (without detector systematics). The GoF in the case without detector systematics has a p-value of 0.33 ($\chi^2/ndf$=43.31/40), showing good agreement between data and model prediction.

Figure 9 shows the comparison between data and prediction as a function of the reconstructed energy of the hadronic system $E^{rec}_{had}$. Left (right) panel is shown with fully systematic uncertainties (without detector systematics). The GoF in the case without detector systematics has a p-value of 0.46 ($\chi^2/ndf$=32.19/32), showing good agreement between data and model prediction. We should further note that the data of the lowest $E^{rec}_{had}$ bin is above the prediction and outside the uncertainty band. Since the $E^{rec}_{had}$ is low for these events, it is natural to raise the question whether the model describes the missing energy because of neutrons or low-energy gammas well. We will come back to this point in the next two sections and show the current model is sufficient in describing the observations in data.

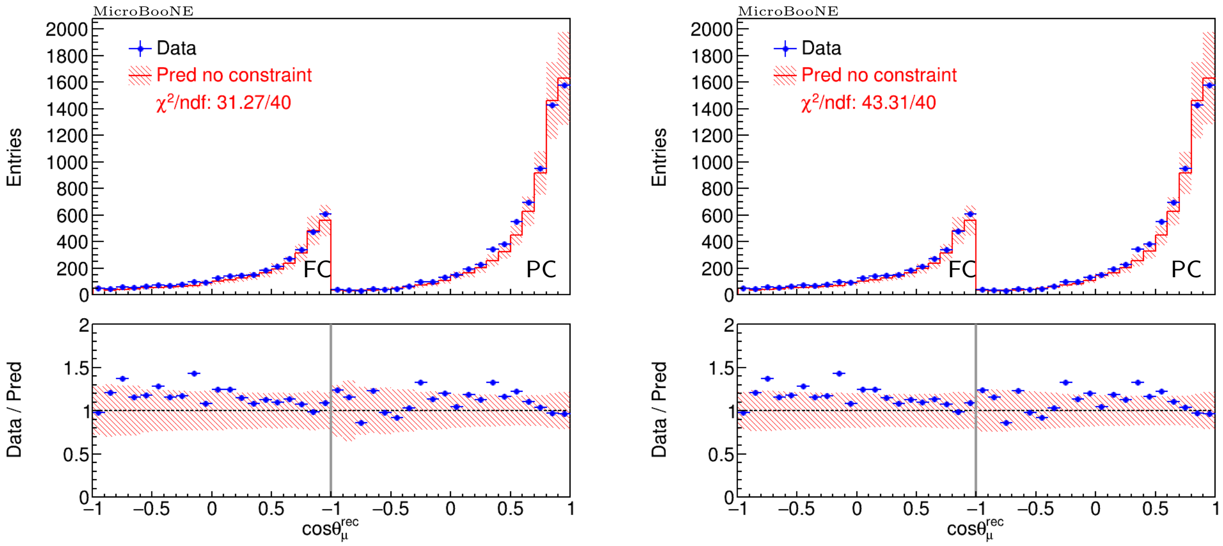


FIG. 8. Comparison between data and prediction as a function of $\cos\theta^{rec}_{\mu}$ (relative to the beam direction): (left) all systematic uncertainties, (right) without detector systematic uncertainties. The statistical uncertainties of the data and Monte Carlo are also included in the bands. For each plot, the first 20 bins correspond to the fully contained events covering from -1 to 1. The next 20 bins correspond to the partially contained events covering from -1 to 1.

Figure 10 shows the comparison between data and prediction as a function of the reconstructed neutrino energy $E^{rec}_{\nu}$. Left (right) panel is shown with full systematic uncertainties (without detector systematics). The GoF in both cases showing good agreement between data and model prediction. The plots shown in this section cover the essential kinematics variables to reconstruct the neutrino energy and the primary muon angle. These comparisons indicate that the model with its associated uncertainties can describe the observations in the data well. Beside these, we have performed data/MC comparison in many kinematics variables including neutrino vertex distribution and azimuthal angle distributions. Overall, good consistencies, measured by the GoF values, are observed. In next two sections, we will use the conditional covariance matrix method to perform more stringent examinations of the overall model.

### D. GoF Tests of PC $\nu_\mu$CC after applying constraints from FC $\nu_\mu$CC: A stringent test of the modeling of the missing energy outside the active TPC volume

For PC events, the reconstructed (neutrino, muon, hadronic) energy only takes into account the visible part of the system inside the active TPC volume. The conversion between the true neutrino energy and the reconstructed neutrino energy thus has stronger dependence on the overall model, which is used to predict the amount of (deposited) energy outside the active TPC volume. Therefore, it is crucial to perform dedicated validations on this part. Since the missing energy (outside the active TPC volume) is invisible by definition, the validation can only be performed on the reconstructed energy. As shown in the previous section, the direct comparison of the PC distributions with the overall model yields good GoF values indicating consistent results. However, these tests include all sources of systematics, which may hide the potential discrepancies on the modeling of missing energy for the PC events. To validate the modeling of the missing energy for the PC events, we perform a more stringent test: calculate GoF of the PC $\nu_\mu$CC distributions after constraining the FC $\nu_\mu$CC distributions following the method outlined in Eq. 4. In this case, the common systematic uncertainties to the PC and FC channels are largely cancelled, and a more stringent validation on the modeling of missing energy of PC events can be achieved.

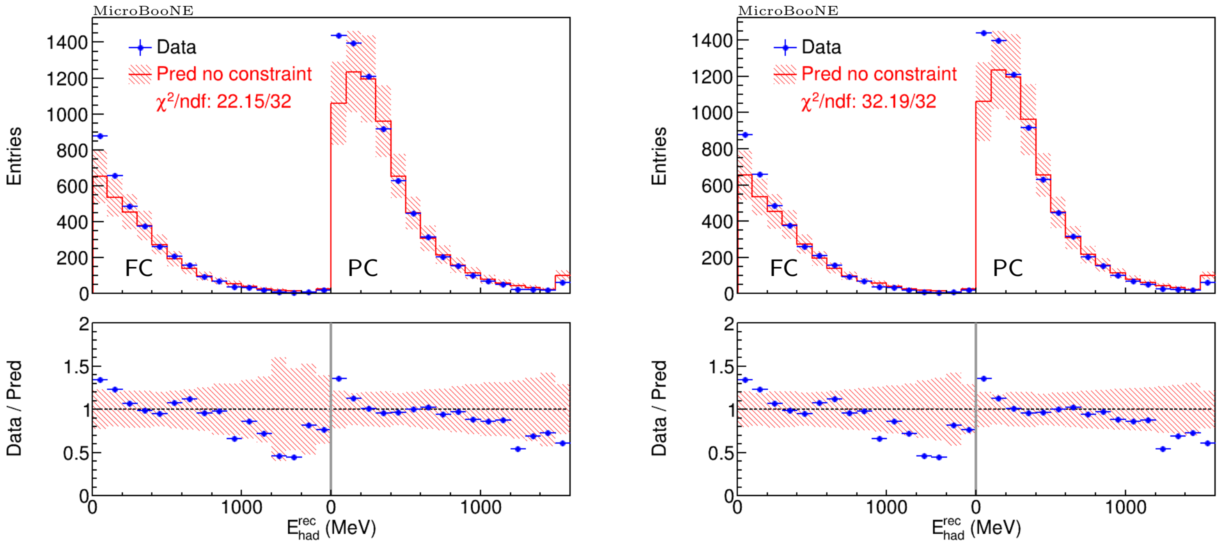


FIG. 9. Comparison between data and prediction as a function of $E_{had}^{rec}$: (left) all systematic uncertainties, (right) without detector systematic uncertainties. The statistical uncertainties of the data and Monte Carlo are also included in the bands. For each plot, the first 15 bins with 100 MeV per bin correspond to the fully contained events from 0 GeV to 1.5 GeV. The 16th bin is the overflow bin corresponding to fully contained events above 1.5 GeV. The next 15 bins with 100 MeV per bin correspond to the partially contained events from 0 GeV to 1.5 GeV. The last bin is the overflow bin corresponding to the partially contained events above 1.5 GeV.

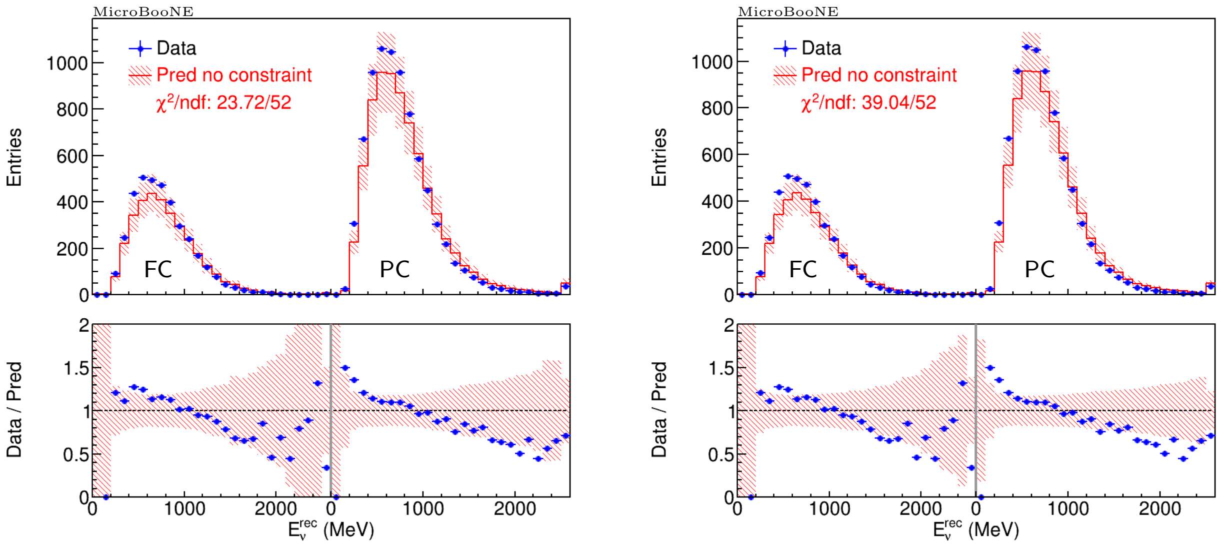


FIG. 10. Comparison between data and prediction as a function of $E_{\nu}^{rec}$: (left) all systematic uncertainties, (right) without detector systematic uncertainties. The statistical uncertainties of the data and Monte Carlo are also included in the bands. For each plot, the first 25 bins with 100 MeV per bin correspond to the fully contained events from 0 GeV to 2.5 GeV. The 26th bin is the overflow bin corresponding to fully contained events above 2.5 GeV. The next 25 bins with 100 MeV per bin correspond to the partially contained events from 0 GeV to 2.5 GeV. The last bin is the overflow bin corresponding to the partially contained events above 2.5 GeV.

Figure 11 shows the comparison between data and prediction as a function of $E_{\mu}^{rec}$ for the PC events. After applying the constraints from the FC sample in $E_{\mu}^{rec}$, the uncertainties of the prediction are significantly reduced. Nevertheless, the GoF values are still reasonable, indicating that the model describes the difference between FC and PC events very well.

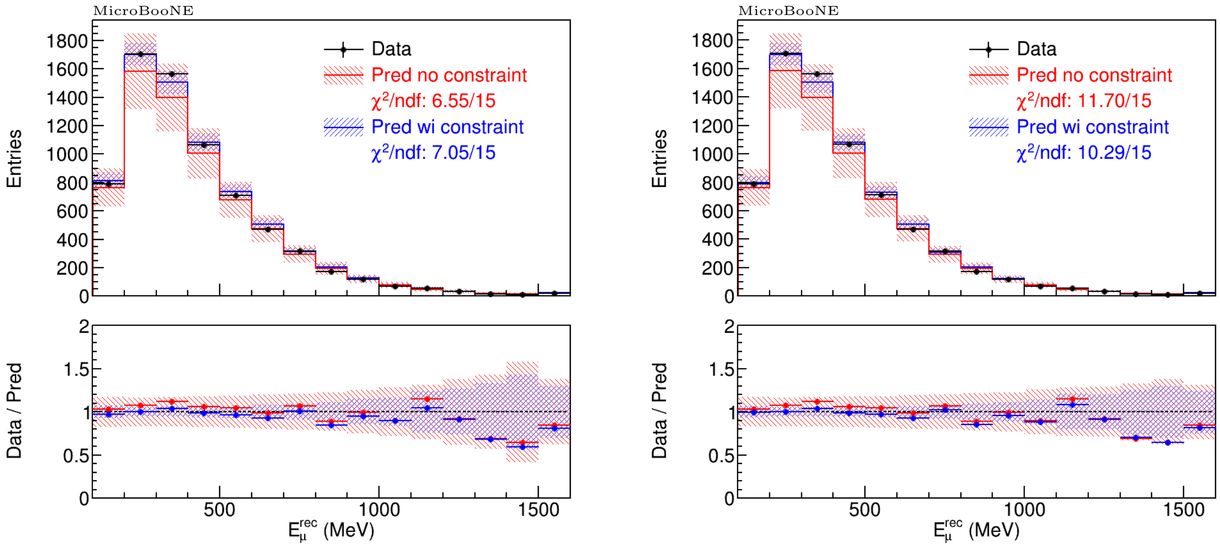


FIG. 11. Comparison between data and prediction as a function of $E_\mu^{rec}$ for the partially contained events: (left) all systematic uncertainties, (right) without detector systematic uncertainties. The red (blue) lines and bands show the prediction without (with) the constraints from the fully contained event sample. The statistical uncertainties of the data and Monte Carlo are also included in the bands. For each plot, the first 14 bins for 100 MeV per bin cover from 0.1 GeV to 1.5 GeV. The last bin is the overflow bin for events above 1.5 GeV.

Figure 12 shows the comparison between data and prediction as a function of $\cos\theta_\mu^{rec}$ for the PC events. After applying the constraints from the FC sample in $\cos\theta_\mu^{rec}$, the uncertainties of the prediction are significantly reduced. Nevertheless, the GoF values (e.g. $\chi^2/ndf = 28.30/20$ with a p-value of 0.10) are still reasonable, indicating that the model describes the difference between FC and PC events well. We should note that at the most forward muon angle, the prediction after constraints is enhanced, which slightly increases the difference between data and prediction. This change is the result of the fact that the data is higher than prediction in this bin for the FC events.

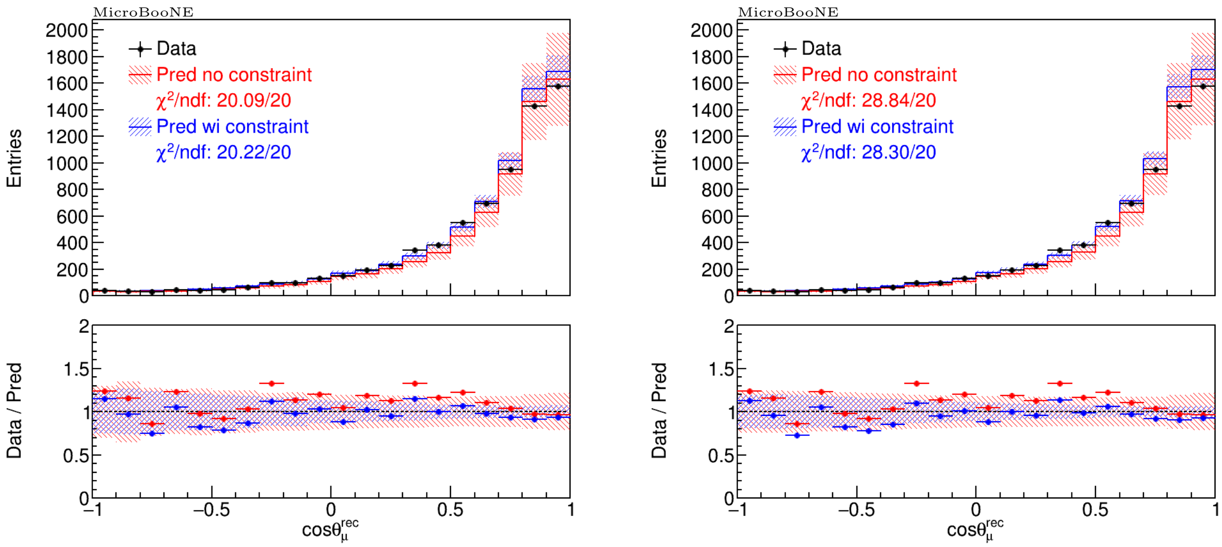


FIG. 12. Comparison between data and prediction as a function of reconstructed muon angle $\cos\theta_\mu^{rec}$ (relative to the beam direction): (left) all systematic uncertainties, (right) without detector systematic uncertainties. The red (blue) lines and bands show the prediction without (with) the constraints from the fully contained event sample. The statistical uncertainties of the data and Monte Carlo are also included in the bands. For each plot, the 20 bins cover from -1 to 1.

Figure 13 shows the comparison between data and prediction as a function of $E_{had}^{rec}$ for the PC events. After applying the constraints from the FC sample in $E_{had}^{rec}$, the uncertainties of the prediction are significantly reduced. Nevertheless, the GoF values are still reasonable indicating the model describes the difference between FC and PC events very well. In particular, we should note the prediction at the lowest bin of $E_{had}^{rec}$ is enhanced after applying the constraints from the FC sample. This is expected since a similar behaviour is observed in the FC sample. Figure 14 shows the comparison between data and prediction as a function of $E_{\nu}^{rec}$ for the PC events. After applying the constraints from the FC sample in $E_{\nu}^{rec}$, the uncertainties of the prediction are significantly reduced. Nevertheless, the GoF values are still reasonable indicating the model describes the difference between FC and PC events very well.

With the results shown in this section, we demonstrate that the model with its associated uncertainties can describe well the difference between the PC and FC events (i.e. the missing energy that is outside the TPC active volume).

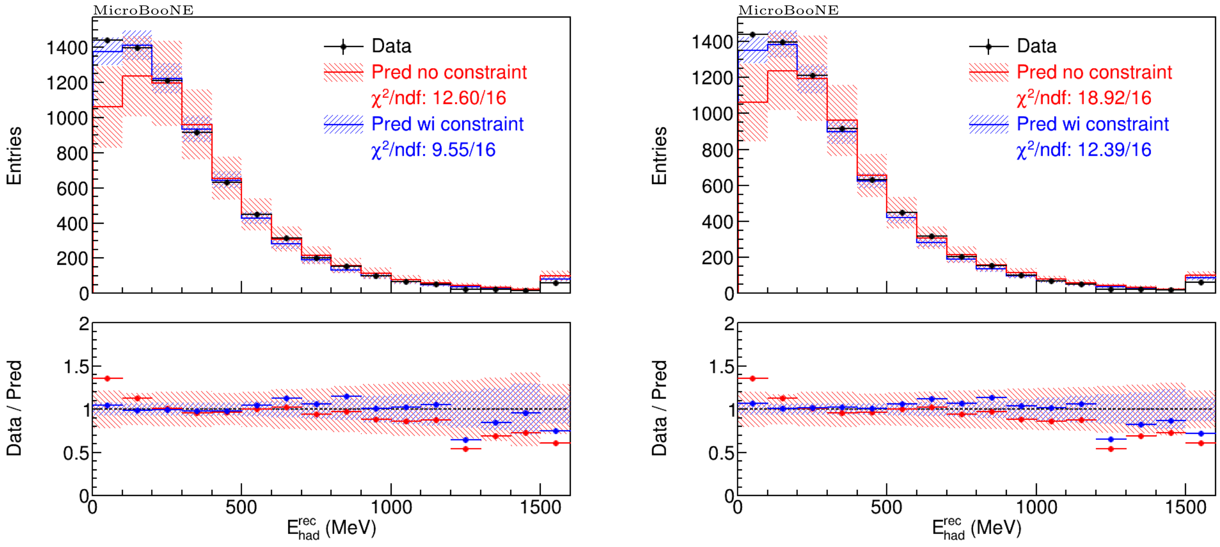


FIG. 13. Comparison between data and prediction as a function of the $E_{had}^{rec}$: (left) all systematic uncertainties, (right) without detector systematic uncertainties. The red (blue) lines and bands show the prediction without (with) the constraints from the fully contained event sample. The statistical uncertainties of the data and Monte Carlo are also included in the bands. For each plot, the first 15 bins correspond to 0 GeV to 1.5 GeV. The last bin correspond to overflow bin above 1.5 GeV.

### E. GoF Tests of $E_{had}$ distribution after applying constraints from muon kinematics for $\nu_\mu$CC: a stringent test of the modeling of the reconstructed neutrino energy

Similar to the situation of PC events, the reconstructed energy of the hadronic system $E_{had}^{rec}$ cannot be directly mapped to the energy transfer to the liquid argon system, since some of the energy going into the neutron and low-energy gamma might be missing. In this case, the map of $E_{had}^{rec}$ to the energy transfer would rely on the overall model, particularly the cross-section model. To validate the modeling of the missing energy in neutrons and low-energy gammas, a similar strategy using the conditional covariance matrix formalism is used. We examine the $E_{had}^{rec}$ distribution after constraining the muon kinematics. In particular, we consider two one-dimensional muon kinematics: $E_{\mu}^{rec}$ and $\theta_{\mu}^{rec}$. For this case, we need to consider the correlation in the statistical covariance matrix in addition to the correlation in the systematic covariance matrix, since the two distributions are coming from the same set of events from the same channel. Such a statistical covariance matrix can be built using the boostrapping method with resampling of the Monte Carlo events.

Figure 15 shows the comparison between data and prediction as a function of $E_{had}^{rec}$ for both FC and PC events. After applying the constraints from the $E_{\mu}^{rec}$ distribution, the uncertainties of the prediction are significantly reduced. Nevertheless, the GoF values improves, indicating that the model describes the relation between $E_{had}^{rec}$ and $E_{\mu}^{rec}$ very well. In particular, we note the prediction at the lowest bin of $E_{had}^{rec}$ is enhanced after applying the constraints from the $E_{\mu}^{rec}$ distribution. In other words, the differences between data and prediction in the $E_{had}^{rec}$ distributions are significantly reduced once the difference between data and prediction in the $E_{\mu}^{rec}$ distributions are eliminated within

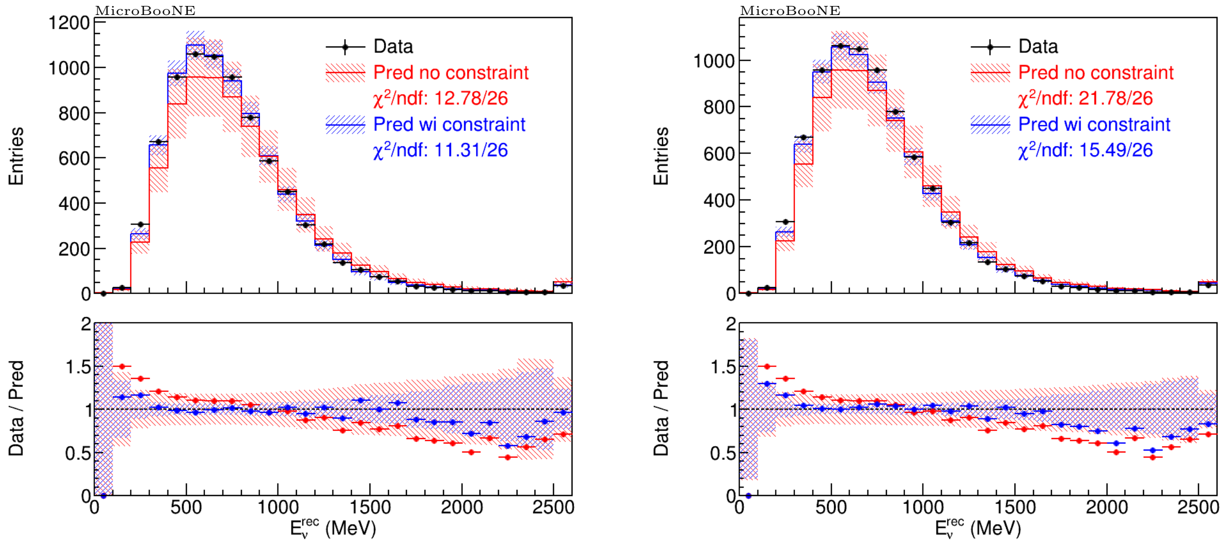


FIG. 14. Comparison between data and prediction as a function of $E_\nu^{rec}$: (left) all systematic uncertainties, (right) without detector systematic uncertainties. The red (blue) lines and bands show the prediction without (with) the constraints from the fully contained event sample. The statistical uncertainties of the data and Monte Carlo are also included in the bands. For each plot, the first 25 bins with 100 MeV per bin correspond to the fully contained events from 0 GeV to 2.5 GeV. The 26th bin is the overflow bin corresponding to fully contained events above 2.5 GeV. The next 25 bins with 100 MeV per bin correspond to the partially contained events from 0 GeV to 2.5 GeV. The last bin is the overflow bin corresponding to the partially contained events above 2.5 GeV.

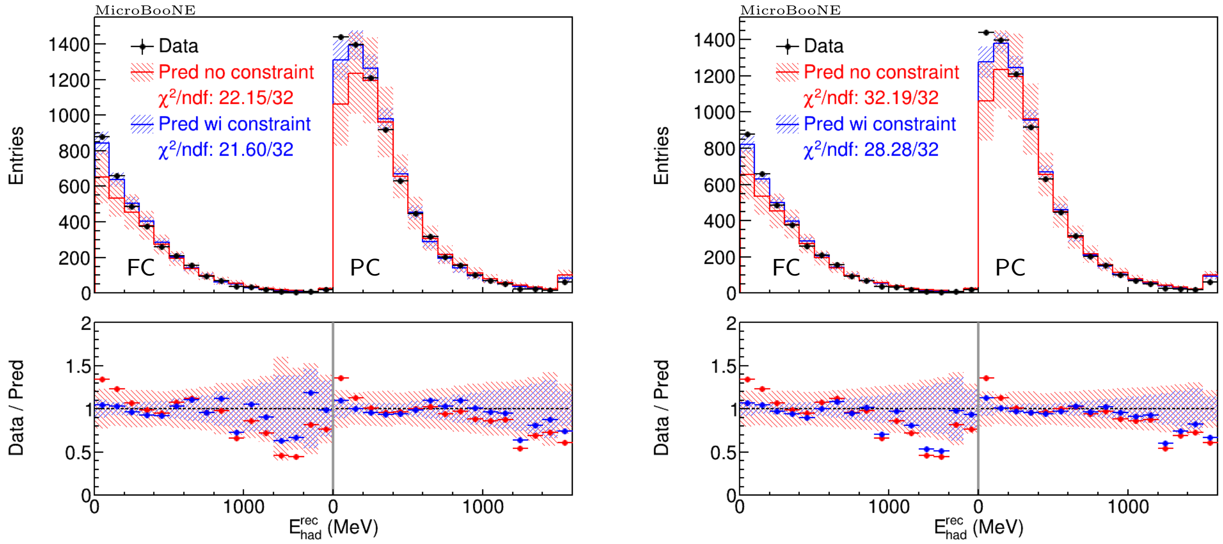


FIG. 15. Comparison between data and prediction as a function of $E_{had}^{rec}$: (left) all systematic uncertainties, (right) without detector systematic uncertainties. The red (blue) lines and bands show the prediction without (with) the constraints from the distributions as a function of $E_\mu^{rec}$. The statistical uncertainties of the data and Monte Carlo are also included in the bands. For each plot, the first 15 bins with 100 MeV per bin correspond to the fully contained events from 0 GeV to 1.5 GeV. The 16th bin is the overflow bin corresponding to fully contained events above 1.5 GeV. The next 15 bins with 100 MeV per bin correspond to the partially contained events from 0 GeV to 1.5 GeV. The last bin is the overflow bin corresponding to the partially contained events above 1.5 GeV.

the allowed range of the model predictions.

To further examine the $E_{had}^{rec}$ distributions, we apply the constraints from the distributions of reconstructed muon angle. First, Fig. 16 shows the comparison between data and prediction as a function of $\cos\theta_\mu^{rec}$ for both FC and PC events. After applying the constraints from the $E_\mu^{rec}$ distribution, the uncertainties of the prediction are significantly reduced. Nevertheless, the GoF values (e.g. $\chi^2/ndf = 44.12/40$ with a p-value of 0.30) improves indicating that the model describes the relation between $\theta_\mu^{rec}$ and $E_\mu^{rec}$ very well. In particular, in the case where the detector systematic uncertainties are removed, the difference between data and predictions at the most forward angle ($\cos\theta_\mu^{rec} \sim 1$) is significantly reduced after applying the constraints from the $E_\mu^{rec}$ distribution. In other words, the differences between data and prediction in the $\cos\theta_\mu^{rec}$ distributions are significantly reduced once the difference between data and prediction in the $E_\mu^{rec}$ distributions are eliminated within the allowed range of the model predictions.

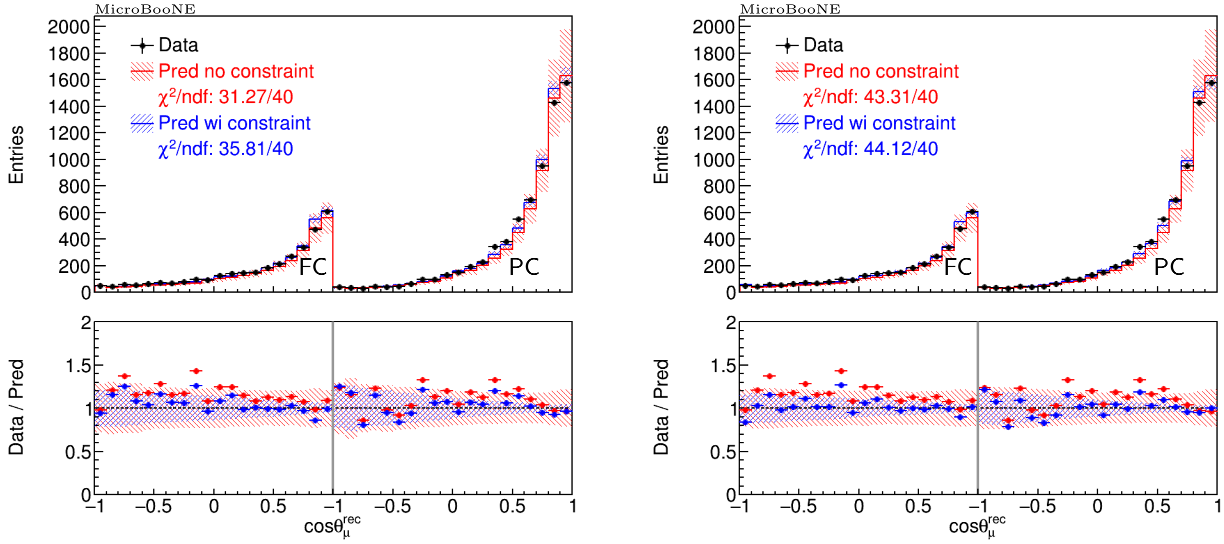


FIG. 16. Comparison between data and prediction as a function of $\cos\theta_\mu^{rec}$ (relative to the beam direction): (left) all systematic uncertainties, (right) without detector systematic uncertainties. The red (blue) lines and bands show the prediction without (with) the constraints from the reconstructed muon energy $E_\mu^{rec}$. The statistical uncertainties of the data and Monte Carlo are also included in the bands. For each plot, the first 20 bins correspond to the fully contained events covering from -1 to 1. The next 20 bins correspond to the partially contained events covering from -1 to 1.

Next, we can add the constraints from the distributions of reconstructed muon angle. Figure 17 shows the comparison between data and prediction as a function of $E_{had}^{rec}$ for both FC and PC events. After applying the constraints from the $E_\mu^{rec}$ and $\cos\theta_\mu^{rec}$ distributions, the uncertainties of the prediction are significantly reduced. Nevertheless, the GoF values improve, indicating that the model describes the relation between $E_{had}^{rec}$ and the muon kinematics very well. In particular, we note the prediction at the lowest bin of $E_{had}^{rec}$ is enhanced after applying the constraints from the $E_\mu^{rec}$ distribution. Compared to Fig. 15, the differences between data and prediction in the lowest bin of $E_{had}^{rec}$ distributions are further reduced by the addition of constraints from reconstructed muon angle.

With results shown in this section, we demonstrate that the model with its associated uncertainties can describe well the difference between $E_{had}^{rec}$ and the energy transferred to the argon nuclei $\nu = E_\nu - E_\mu$ (i.e. the missing energy associated with neutrons and low-energy gamma). We further elaborate on this point below. At the fixed true neutrino energy, the energy transferred to the argon nuclei is associated with the muon kinematics. If the modeling of the missing energy (due to neutrons and low-energy gammas) including its uncertainties is incorrect, one would expect to see significant differences between data and predictions on the $E_{had}^{rec}$ distributions after applying the constraints on the muon kinematics, since this would remove numerous systematic uncertainties in common between these two measurements. Because we did not see such discrepancies in the $E_{had}^{rec}$ distributions after applying constraints on the muon kinematics, we conclude that the current modeling of the missing energy due to neutrons and low-energy gammas is sufficient. While the GoF tests shown are performed with the $5.3{\times}10^{19}$ POT data, the same tests were repeated with a much larger data set ($6.4{\times}10^{20}$ POT) and the same conclusions were obtained. In Sec. IV, we apply these GoF tests to some fake data, which further demonstrates that these tests are stringent in validating the overall model.

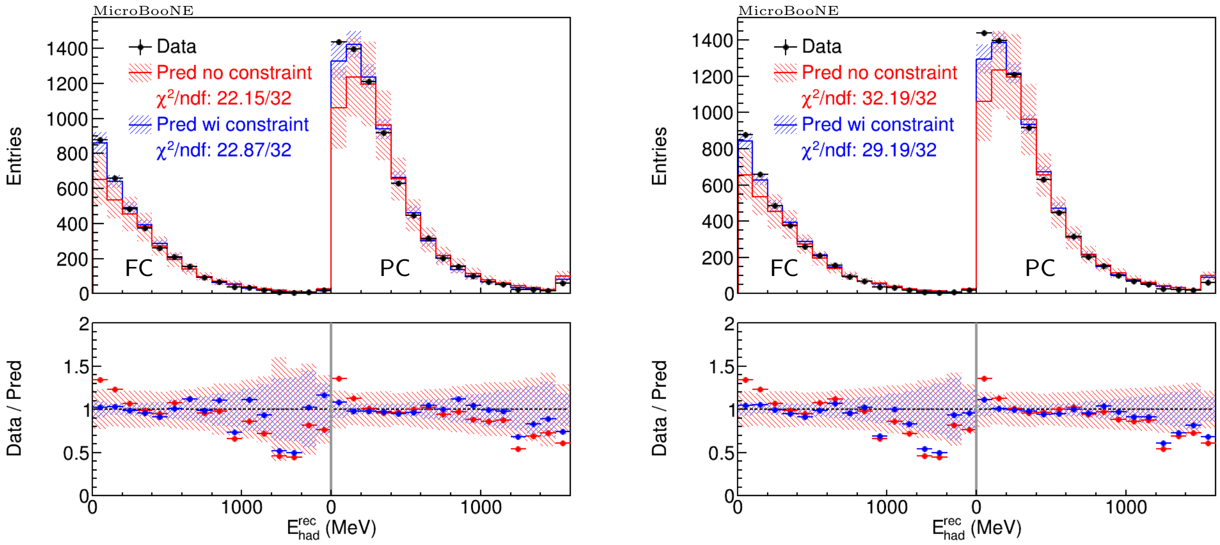


FIG. 17. Comparison between data and prediction as a function of $E^{rec}_{had}$: (left) all systematic uncertainties, (right) without detector systematic uncertainties. The red (blue) lines and bands show the prediction without (with) the constraints from the reconstructed muon energy $E^{rec}_{\mu}$ and angle $\cos\theta^{rec}_{\mu}$. The statistical uncertainties of the data and Monte Carlo are also included in the bands. For each plot, the first 15 bins with 100 MeV per bin correspond to the fully contained events from 0 GeV to 1.5 GeV. The 16th bin is the overflow bin corresponding to fully contained events above 1.5 GeV. The next 15 bins with 100 MeV per bin correspond to the partially contained events from 0 GeV to 1.5 GeV. The last bin is the overflow bin corresponding to the partially contained events above 1.5 GeV.

## III. DESCRIPTIONS OF VARIOUS EVENT GENERATORS

This section briefly introduces the model configurations used in different event generator predictions included in this analysis.

- GENIE v3.0.6: The G18_10a_02_11a model configuration is used. This includes the local Fermi gas model [4] of the nuclear ground state, the Valencia treatment of charged-current QE and 2p2h processes, the KLN-BS RES [5–8] and BS COH [9] scattering models, and the hA2018 FSI model [10].

- MicroBooNE MC (MicroBooNE GENIE Tune): A MicroBooNE-specific modification of the GENIE v3.0.6 model described above. Four model parameters are tuned based on a fit to CC0$\pi$ cross-section data obtained by the T2K experiment [11]. For CCQE events, the nucleon axial mass and strength of the Random Phase Approximation corrections considered in the Valencia model were varied in the fit. For CC 2p2h events, the overall normalization and the shape of the leptonic differential cross section were adjusted. Further details are available in a forthcoming publication.

- "GENIE v2 tune1" (underlying true model for fake dataset): GENIE v2.12.2 [12, 13] with the Bodek-Ritchie Fermi Gas model, the Llewellyn-Smith CCQE scattering prescription [14], and the empirical meson exchange current (MEC) model [15], a Rein-Sehgal resonance (RES) and coherent scattering (COH) model [16], and a data driven final state interaction (FSI) model denoted as "hA" [17].

- NuWro 19.02.1 [18]: Using the Local Fermi Gas model [4], the Llewellyn-Smith CCQE scattering prescription [14], the Nieves MEC model [19], the Adler-Rarita-Schwinger formalism to calculate the $\Delta$ resonance explicitly [20], the BS COH [9] scattering model and an intranuclear cascade model for FSI.

- NEUT v5.4.0 [21]: Using the Local Fermi Gas model [4], the Nieves CCQE scattering prescription [22], the Nieves MEC model [19], the BS RES [5–8] and Rein-Sehgal COH [9] scattering models, and FSI with Oset medium correction for pions [23].

- GiBUU 2019 [24]: Using somewhat similar models, but unlike in other generators, those are implemented in a coherent way, by solving the Boltzmann-Uehling-Uhlenbeck transport equation. The models include: Local

Fermi Gas model [4], standard CCQE expression [25], empirical MEC model and a dedicated spin-dependent resonances amplitude calculation following the MAID analysis [26]. The DIS model is as in PYTHIA [27] and the FSI treatment is different as the hadrons propagate through the residual nucleus, in a nuclear potential which is consistent with the initial state.

## IV. FAKE DATA STUDY

We have carried out a dedicated study with fake data to demonstrate the validity of our procedure in examining the overall model (e.g. characterizing the mapping between the true neutrino energy and the reconstructed neutrino energy) and extracting the cross section as a function of the neutrino energy.

### A. A Sanity Check: Fake data with GENIE v3 model

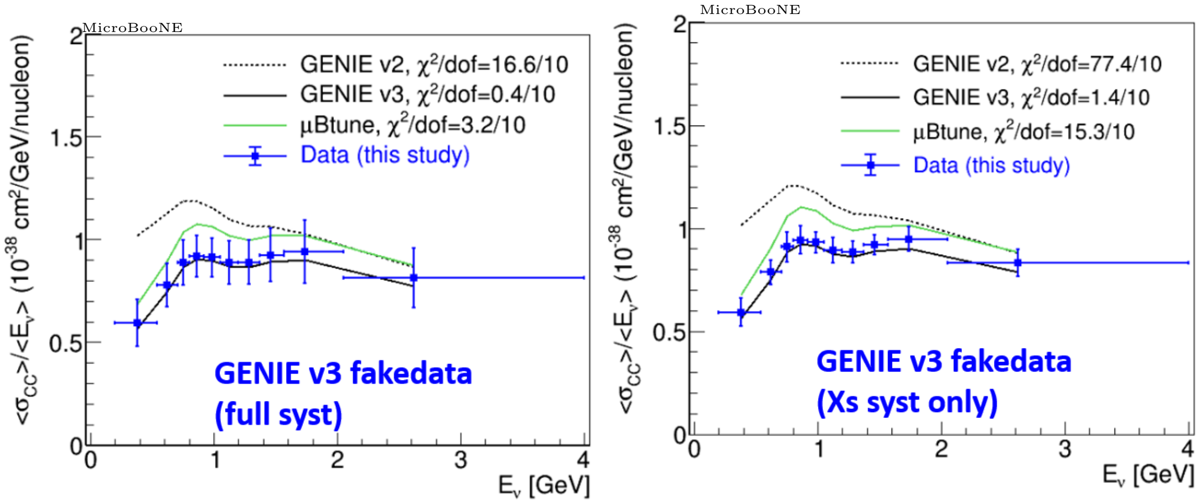


FIG. 18. Extracted total cross section (per nucleon) normalized by energy as a function of neutrino energy for the GENIE-v3 fake data: (left) considering full systematic uncertainties, and (right) considering cross-section uncertainty only since only the cross-section model is changed in generating this fake data. Three model predictions including GENIE v2, GENIE v3, and $\mu$B Tuned (nominal Monte Carlo simulation) are shown. More details about these models can be found in Sec. III. The goodness-of-fit $\chi^2/ndf$ for each model is shown. As expected, the GoF value for the GENIE v3, which is the truth of the fake data, is the smallest.

We constructed a fake data set at $5.3\times10^{19}$ POT using the standard GENIE v3 model [28] by removing the additional event weights of the MicroBooNE tune using the standard Monte Carlo events. As shown in Fig. 18, the extracted cross section is most consistent with the underlying true model (GENIE v3) with the smallest (and close-to-zero) $\chi^2/ndf$. The non-zero $\chi^2/ndf$ is the result of constructing the overall response matrix with the standard MicroBooNE Monte Carlo ($\mu$Btune), which is slightly different from that of the GENIE v3 model. We should note that the statistical fluctuation in this fake data set is small compared to the overall systematic uncertainties. At the same time, the close-to-zero $\chi^2/ndf$ indicates the high similarity between the truth (GENIE v3) and the Monte Carlo simulation (GENIE v3 with MicroBooNE tune). The analysis of this fake data set essentially serves as a sanity check of the cross-section extraction procedure.

### B. Test of Model Validations: Fake data with GENIE v2 model

A set of fake data is generated with the GENIE v2 model with a $7.2\times10^{20}$ POT exposure. Given that the underlying cross-section models are quite different between the GENIE v2 and GENIE v3 models, we not only can use this fake data to demonstrate validity of the cross-section extraction, but can also use this fake data to demonstrate the effectiveness of the model validations. In particular, we repeated the study of GoF tests of $E_{had}$ distribution after applying constraints from muon kinematics (Sec. II E). Figure 19 shows the data/MC comparison in $E_{had}^{rec}$ before

and after applying the constraints from muon kinematics. While the data is consistent with the model prior to the application of the constraints, the data is NOT consistent with the model after applying the constraints from the muon kinematics. The $\chi^2/ndf$ value in the latter case is 116.9/32, giving a p-value of $1.338\times10^{-11}$. This demonstrates that if the GENIE v2 cross-section model is true, the overall MicroBooNE model built upon the GENIE v3 model is NOT consistent with the modeling of missing energy in GENIE v2 cross-section model. In comparison, the same study done in Sec. II E gives a $\chi^2/ndf$ value of 29.2/32 (p-value of 0.61) when comparing data with the MC prediction in $E^{rec}_{had}$ after applying the constraints from the muon kinematics. The same conclusion remains when we analyze a much larger data set at $6.4\times10^{20}$ POT. This test again confirms that the overall MicroBooNE model is consistent with the real data with respect to the modeling of missing energy.

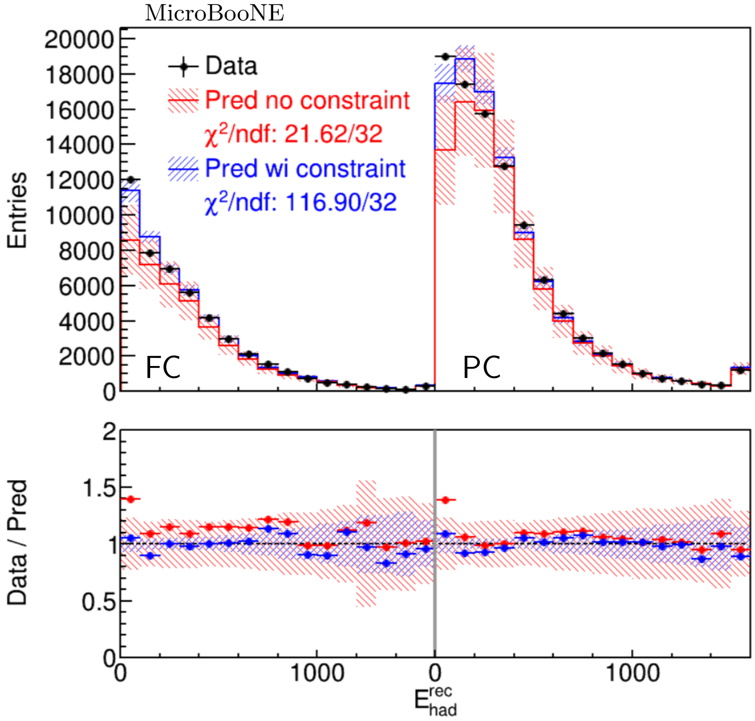


FIG. 19. Comparison between data and prediction as a function of $E^{rec}_{had}$: all systematic uncertainties included. The red (blue) lines and bands show the prediction without (with) the constraints from the reconstructed muon energy $E^{rec}_{\mu}$ and angle $\cos\theta^{rec}_{\mu}$. The statistical uncertainties of the data and Monte Carlo are also included in the bands. For each plot, the first 15 bins with 100 MeV per bin correspond to the fully contained events from 0 GeV to 1.5 GeV. The 16th bin is the overflow bin corresponding to fully contained events above 1.5 GeV. The next 15 bins with 100 MeV per bin correspond to the partially contained events from 0 GeV to 1.5 GeV. The last bin is the overflow bin corresponding to the partially contained events above 1.5 GeV.

Although the previous test has shown that the fake data set with GENIE v2 model is not compatible with our overall model with its uncertainties, we proceeded ahead to extract the total cross section as function of neutrino energy. The left panel of Fig. 20 shows the extracted total cross section per nucleon after normalizing by the the neutrino energy. The extracted total cross-section points are consistent with the truth information (GENIE v2) within 1 $\sigma$. The overall goodness-of-fit value, which considers the full correlations of the uncertainties, gives the smallest goodness-of-fit value $\chi^2/ndf = 5.7/10$ (i.e. p-value of 0.84) for GENIE v2 among three models: GENIE v2, GENIE v3, and MicroBooNE Tune.

Since only the cross-section model is changed in generating this fake data, we repeat the above study by only considering the systematic uncertainties from cross section in addition to the Monte Carlo statistics. In other words, we exclude the systematic uncertainties from the neutrino flux, GEANT4, and detector systematics. The right panel of Fig. 20 shows the thus extracted total cross section per nucleon normalized by neutrino energy. Compared to the results shown in the left panel, the uncertainties of the unfolded cross section become smaller as expected. Compared to the truth information, many of the points are now outside the 1$\sigma$ error band. However, the goodness-of-fit test considering the correlated uncertainties in the unfolded cross section still yields the smallest GoF value $\chi^2/ndf = 11/10$ (i.e. p-value of 0.36) among three models: GENIE v2, GENIE v3, and MicroBooNE Tuned. The decent p-value of 0.36 indicates that the unfolded cross-section results are consistent with the truth information. This demonstrates the validity of the cross-section extraction procedure despite the fact that this fake data is not consistent with our

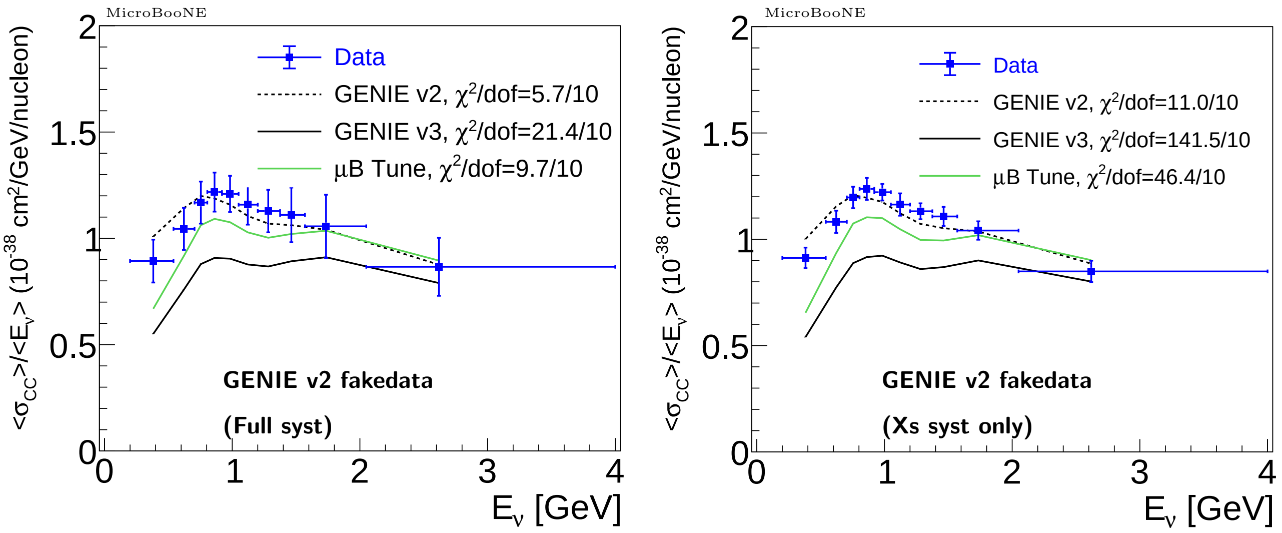


FIG. 20. Total cross sections (per nucleon) normalized by neutrino energy as a function of neutrino energy are extracted: (left) with full systematic uncertainties, (right) with only the cross-section uncertainty considered in addition to the MC statistics and data statistical uncertainties. Three model predictions including GENIE v2, GENIE v3, and $\mu$B Tune (nominal Monte Carlo simulation) are shown. The goodness-of-fit $\chi^2/ndf$ for each model is shown. As expected, the GoF value for the GENIE v2, which is the truth of the fake data, is the smallest in both cases.

overall model within its uncertainties. This means that the validation of the neutrino energy reconstruction using the conditional covariance method (particularly examining the data/MC comparison of $E^{rec}_{had}$ after applying the constraints on muon kinematics) is more stringent than the total cross-section unfolding procedure.

### C. Quantification of the neutrino energy reconstruction: Fake data with GENIE v3 and MicroBooNE Tune by altering reconstructed energy of protons

In the previous section, through analyzing the fake data with GENIE v2, we showed that the validation of the neutrino energy reconstruction using the conditional covariance method (particularly examining the data/MC comparison of $E^{rec}_{had}$ after applying the constraints on muon kinematics) is more stringent than the total cross-section unfolding procedure. In order to quantify the sensitivity of the conditional covariance method to the missing energy (e.g. neutrons or low-energy gammas), we create a new fake data set by reducing the reconstructed proton energy, which mimics a realistic systematic effect whereby more visible energy (e.g. from protons) could become invisible (e.g. neutrons) especially in the hadronic final states. The nominal Monte-Carlo simulations based on GENIE v3 and MicroBooNE Tune is used to generate this set of fake data. Figure 21 shows the energy spectra for different proton energy scaling factors. With a smaller scaling factor, more visible energy become invisible and the energy spectrum become softer as expected.

The additional invisible energy introduced to the hadronic system can be quantitatively expressed by the mean fraction of additional invisible energy relative to the true energy transfer, as a function of true neutrino energy. Fig. 22 shows the mean fraction of additional invisible energy we introduced on top of the nominal Monte-Carlo (MicroBooNE GENIE tune). The new fake data sets adequately cover the variation of NEUT and GENIE generator central values.

Following the same procedure reported in Sec. II E, a conditional GoF test of $E^{rec}_{had}$ after constraint from $E_\mu$ and muon cos$\theta$ measurements is performed for each new fake data sample with different $E^{rec}_p$ scaling factors. The $\chi^2$ values (Pearson) and p-values (assuming standard $\chi^2$ distributions in each case) are summarized in Tab. I. The results when considering cross-section systematic alone are shown in Tab. II. With total (cross-section only) systematic uncertainties included, the conditional GoF test can clearly detect scaling factor of 0.7 (0.85), which corresponds to 30% (or 15%) additional missing energy.

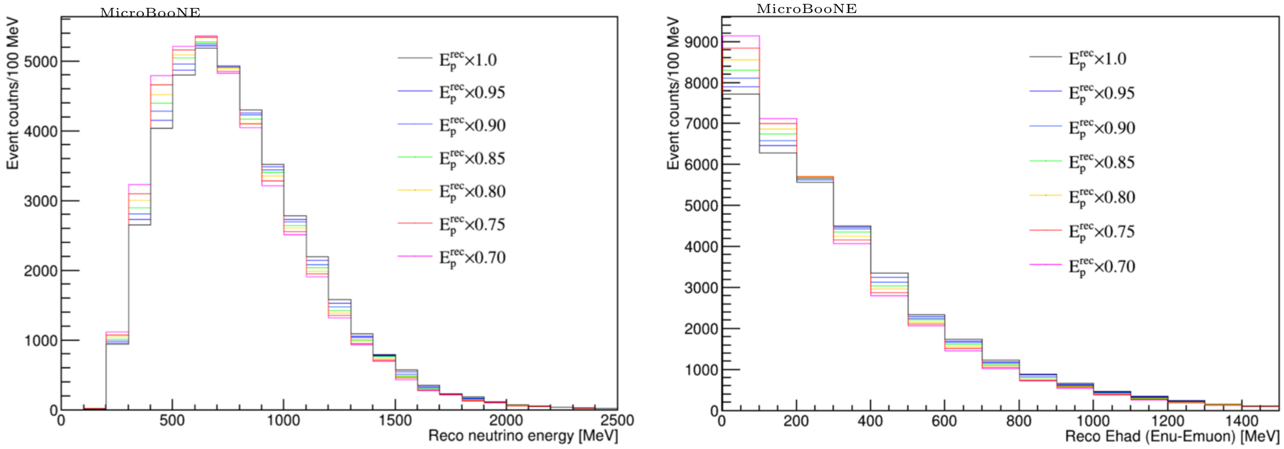


FIG. 21. Spectra of reconstructed neutrino energy $E_\nu^{rec}$ (left) and hadronic energy $E_{had}^{rec}$ (right, $E_\nu^{rec}$-$E_\mu^{rec}$) for the new fake data samples. With a smaller scaling factor, the energy spectrum is softer.

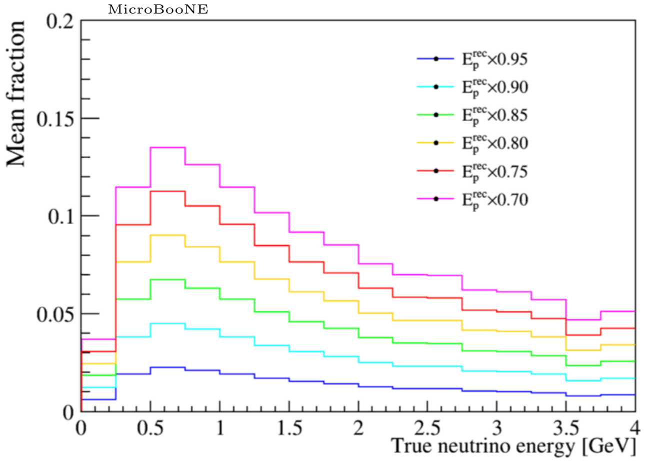


FIG. 22. Mean fraction of additional invisible energy relative to true energy transfer as a function of true neutrino energy. Each curve corresponds to a different scaling factor on reconstructed proton energy for those selected $\nu_\mu$CC events, showing a variation of invisible energy on top of the Monte-Carlo central values.

| $E_p^{rec}$ scaling factor | FC events (ndf=16) | PC events (ndf=16) | FC+PC (ndf=32) |
|---|---|---|---|
| 0.95 | 0.62 (1.00) | 1.10 (1.00) | 1.58 (1.00) |
| 0.90 | 2.05 (1.00) | 4.63 (1.00) | 6.24 (1.00) |
| 0.85 | 4.37 (1.00) | 10.78 (0.82) | 14.36 (1.00) |
| 0.80 | 7.41 (0.96) | 18.72 (0.28) | 24.58 (0.82) |
| 0.75 | 11.31 (0.79) | 29.10 (0.02) | 37.86 (0.22) |
| 0.70 | 15.39 (0.50) | 41.73 (0.00) | 53.85 (0.01) |

TABLE I. $\chi^2$ and p-value (in the parentheses) considering full systematic uncertainty for $E_{had}^{rec}$ data/MC comparisons after constraint from $E_\mu$ and muon $\cos\theta$ measurements. Each row corresponds to a different scaling factor which is quantitatively interpreted in Fig. 22.

| $E_p^{rec}$ scaling factor | FC events (ndf=16) | PC events (ndf=16) | FC+PC (ndf=32) |
|---|---|---|---|
| 0.95 | 2.55 (1.00) | 4.08 (1.00) | 5.34 (1.00) |
| 0.90 | 8.90 (0.92) | 17.13 (0.38) | 21.05 (0.93) |
| 0.85 | 18.66 (0.29) | 39.45 (0.00) | 47.01 (0.04) |
| 0.80 | 32.95 (0.01) | 67.88 (0.00) | 80.60 (0.00) |

TABLE II. $\chi^2$ and p-value (in the parentheses) considering cross-section only systematic uncertainty for $E_{had}^{rec}$ data/MC comparisons after constraint from $E_\mu$ and muon $\cos\theta$ measurements. Each row corresponds to a different scaling factor which is quantitatively interpreted in Fig. 22.

Figure 23 shows the extracted total cross section as a function of neutrino energy for fake data where the proton energies are scaled by 0.85. Even in the case that only cross-section uncertainties are considered, the GoF value after adjustment for potential statistical fluctuation and systematic variation $\chi^2/ndf = (4.1 + 10)/10$ is quite reasonable. Given that the conditional constraining check has detected that a 15% of the energy shift in the proton energy is outside the allowed region of cross-section systematic uncertainties, we confirmed the earlier conclusion that the validation of the neutrino energy reconstruction using the conditional covariance method is more stringent than the total cross-section unfolding procedure.

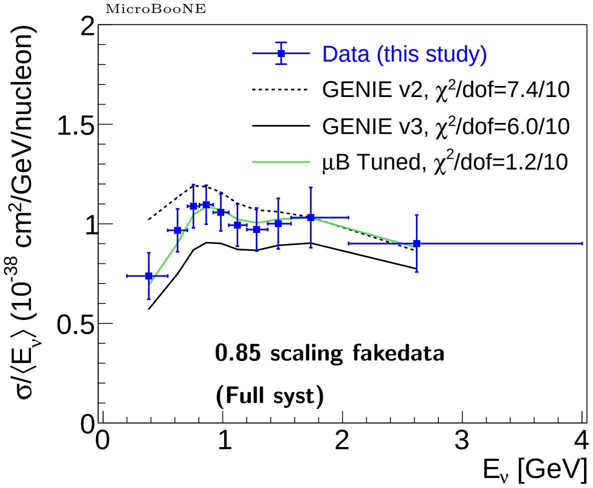


FIG. 23. Extracted total cross sections (per nucleon) normalized by neutrino energy as a function of neutrino energy are shown. Proton energies are scaled by 0.85. Full systematic uncertainties are considered. Three model predictions including GENIE v2, GENIE v3, and $\mu$B Tuned (nominal Monte Carlo simulation) are shown. The goodness-of-fit $\chi^2/ndf$ for each model is shown.

Figure 24 shows the extracted total cross section as a function of neutrino energy for a fake data set where the proton energies are scaled by 0.7. In the case where full systematic uncertainties are considered, the GoF value after adjustment for potential statistical fluctuation and systematic variation $\chi^2/ndf = (5.2 + 10)/10$ is quite reasonable. Given the conditional constraining check has detected that a 30% of the energy shift in the proton energy is outside the allowed region of full systematic uncertainties, we again confirmed the earlier conclusion that the validation of the neutrino energy reconstruction using the conditional covariance method is more stringent than the total cross-section unfolding procedure.

## V. FORMATION OF MASTER EQUATION TO UNFOLD TOTAL CROSS SECTION AS A FUNCTION OF NEUTRINO ENERGY

The process of extracting information about the truth content of the measurement bins, given the observed measurements, is referred to as "unfolding." For a typical data unfolding problem, the formation of the master equation

$$M = R \cdot S \tag{6}$$

is crucial. Here $M$ is the measurable quantity (typically a vector) in the reconstructed kinematics variable space. $S$ is the physics quantity (typically also a vector) to be extracted in the true kinematics variable space, which is the goal

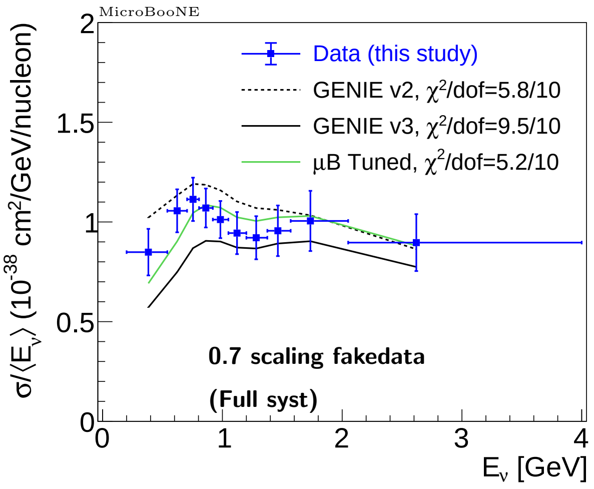


FIG. 24. Extracted total cross sections (per nucleon) normalized by neutrino energy as a function of neutrino energy are shown. Proton energies are scaled by 0.7. Full systematic uncertainties are considered. Three model predictions including GENIE v2, GENIE v3, and $\mu$B Tuned (nominal Monte Carlo simulation) are shown. The goodness-of-fit $\chi^2/ndf$ for each model is shown.

of the unfolding procedure. Then $R$, which is assumed to be known, is a matrix connecting the unknown $S$ with the actual measurement $M$, and can be determined from theoretical modeling or Monte Carlo (MC) simulation.

In the case of the cross section as a function of energy, $M$ represents the measured number of events as a function of the reconstructed neutrino energy $E_{rec}$:

$$M(E_{rec}) = POT \cdot T \cdot \int F(E_\nu) \cdot \sigma(E_\nu) \cdot D(E_\nu, E_{rec}) \cdot \epsilon(E_\nu, E_{rec}) \cdot dE_\nu + B(E_{rec}), \tag{7}$$

Here, $POT$ and $T$ represent the integrated proton-on-target and the number of target nucleons. $F(E_\nu)$ is the muon neutrino flux as a function of the true neutrino energy $E_\nu$. $\sigma(E_\nu)$ is the total $\nu_\mu$CC interaction cross section as a function of the true neutrino energy $E_\nu$. $D(E_\nu, E_{rec})$, the detector response matrix, is a function of both the $E_\nu$ and $E_{rec}$, and it represents the smearing of the neutrino energy reconstruction. $\epsilon(E_\nu, E_{rec})$, which is also a function of both the $E_\nu$ and $E_{rec}$, represents the selection efficiency. The last term, $B(E_{rec})$, represents the estimation of backgrounds as a function of $E_{rec}$, which also depends on the $POT$, $T$, $F$, $\sigma$, as well as the selection strategy.

We can rewrite Eq. (7) in a matrix format:

$$M_i = \sum_j \widetilde{S}_{ij} + B_i, \tag{8}$$

with $i$ is the bin in the $E_{rec}$ and $j$ is the bin in $E_\nu$ and

$$\begin{aligned} \widetilde{S}_{ij} &= \frac{POT \cdot T \cdot \int_j F(E_{\nu\ j}) \cdot \sigma(E_{\nu\ j}) \cdot D(E_{\nu\ j}, E_{rec\ i}) \cdot \epsilon(E_{\nu\ j}, E_{rec\ i}) \cdot dE_{\nu\ j}}{POT \cdot T \cdot \int_j \overline{F}(E_{\nu\ j}) \cdot \sigma(E_{\nu\ j}) \cdot dE_{\nu\ j}} \\ &\cdot \left(POT \cdot T \cdot \int_j \overline{F}(E_{\nu\ j}) \cdot dE_{\nu\ j}\right) \cdot \frac{\int_j \overline{F}(E_{\nu\ j}) \cdot \sigma(E_{\nu\ j}) \cdot dE_{\nu\ j}}{\int_j \overline{F}(E_{\nu\ j}) \cdot dE_{\nu\ j}} \\ &= \widetilde{\Delta}_{ij} \cdot \widetilde{F}_j \cdot S_j, \end{aligned} \tag{9}$$

with

$$\widetilde{\Delta}_{ij} \equiv \frac{POT \cdot T \cdot \int_j F(E_{\nu\ j}) \cdot \sigma(E_{\nu\ j}) \cdot D(E_{\nu\ j}, E_{rec\ i}) \cdot \epsilon(E_{\nu\ j}, E_{rec\ i}) \cdot dE_{\nu\ j}}{POT \cdot T \cdot \int_j \overline{F}(E_{\nu\ j}) \cdot \sigma(E_{\nu\ j}) \cdot dE_{\nu\ j}} \tag{10}$$

being the main smearing matrix that can be directly extracted from the Monte Carlo simulation:

$$\widetilde{\Delta}_{ij} = \frac{(\text{Selected no. of events in reco. energy bin i from true energy bin j after event weights})}{(\text{Generated no. of events in true energy bin j after event weights})}, \tag{11}$$

which is also used to estimate the impact of various systematic uncertainties (e.g. neutrino flux, neutrino-argon interaction cross section, and detector systematics). Here $\overline{F}$ represents the nominal (or central value) of the $\nu_\mu$ neutrino flux. Furthermore,

$$\widetilde{F}_j \equiv POT \cdot T \cdot \int_j \overline{F}\left(E_{\nu\ j}\right) \cdot dE_{\nu\ j} \tag{12}$$

is a constant that can be calculated externally knowing the nominal $\nu_\mu$ neutrino flux and

$$S_j \equiv \frac{\int_j \overline{F}\left(E_{\nu\ j}\right) \cdot \sigma\left(E_{\nu\ j}\right) \cdot dE_{\nu\ j}}{\int_j \overline{F}\left(E_{\nu\ j}\right) \cdot dE_{\nu\ j}}, \tag{13}$$

is the (nominal) flux-averaged total cross section of the true neutrino energy bin $j$ that we pursue in the unfolding procedure. Mapping $R_{ij} = \widetilde{\Delta}_{ij} \cdot \widetilde{F}_j$ to Eq. (8), we have

$$M_i - B_i = \sum_j R_{ij} \cdot S_j, \tag{14}$$

which is essentially the master equation in Eq. (6). It is worth noting that such definition of the extracted cross section is based on the nominal neutrino flux, therefore, it does not explicitly rely on a prior-knowledge of the flux shape uncertainty. All the flux uncertainties enter into the response matrix, and therefore, have been precisely considered in the full covariance matrix. This is consistent with one recommendation in Ref. [29].

## VI. FORMATION OF MASTER EQUATION TO UNFOLD DIFFERENTIAL CROSS SECTIONS

In this section, we describe the exact formalism to form the master equation (Eq. 6) for the extraction of the differential cross section on any kinematics variable $K$. The $M$ represents the measured number of events as a function of the reconstructed kinematics variable $K_{rec}$:

$$M\left(K_{rec}\right) = POT \cdot T \cdot \int\int F\left(E_\nu\right) \cdot \frac{d\sigma\left(E_\nu, K_{true}\right)}{dK_{true}} \cdot D \cdot \epsilon \cdot dE_\nu \cdot dK_{true} + B\left(K_{rec}\right), \tag{15}$$

As before, $POT$ and $T$ represent the integrated protons on target and the number of target nucleons. $F\left(E_\nu\right)$ is the muon neutrino flux as a function of the true neutrino energy $E_\nu$. $\frac{d\sigma(E_\nu, K_{true})}{dK_{true}}$ is the differential cross section as a function of the true neutrino energy $E_\nu$ and $K_{true}$. $D$ (or $D\left(E_\nu, K_{true}, K_{rec}\right)$), the detector response matrix, is a function of the $E_\nu$, $K_{true}$ and $K_{rec}$, and it represents the smearing of the neutrino energy reconstruction. $\epsilon$ (or $\epsilon(E_\nu, K_{true}, K_{rec})$), which is also a function of the $E_\nu$, $K_{true}$, and $K_{rec}$, represents the selection efficiency. The last term, $B\left(K_{rec}\right)$, represents the estimation of backgrounds as a function of $K_{rec}$, which also depends on the $POT$, $T$, $F$, $\sigma$, as well as the selection strategy.

We can rewrite Eq. (15) in a matrix format:

$$M_i = \sum_j \widetilde{S}_{ij} + B_i, \tag{16}$$

where $i$ is the bin in the $K_{rec}$ and $j$ is the bin in $K_{true}$ and

$$\begin{aligned}
\widetilde{S}_{ij} = & \frac{POT \cdot T \cdot \int_j \int F\left(E_\nu\right) \cdot \frac{d\sigma(E_\nu, K_{true\ j})}{dK_{true\ j}} \cdot D\left(E_\nu, K_{true\ j} K_{rec\ i}\right) \cdot \epsilon(E_\nu, K_{true\ j}, K_{rec\ i}) \cdot dE_\nu \cdot dK_{true\ j}}{POT \cdot T \cdot \int_j \int \overline{F}\left(E_\nu\right) \cdot \frac{d\sigma(E_\nu, K_{true\ j})}{dK_{true\ j}} \cdot dE_\nu \cdot dK_{true\ j}} \\
& \cdot \left(POT \cdot T \cdot \int_j \int \overline{F}\left(E_\nu\right) \cdot dE_\nu \cdot dK_{true\ j}\right) \cdot \frac{\int_j \int \overline{F}\left(E_\nu\right) \cdot \frac{d\sigma(E_\nu, K_{true\ j})}{dK_{true\ j}} \cdot dE_\nu \cdot dK_{true\ j}}{\int_j \int \overline{F}\left(E_\nu\right) \cdot dE_\nu \cdot dK_{true\ j}} \\
& = \widetilde{\Delta}_{ij} \cdot \widetilde{F}_j \cdot S_j,
\end{aligned} \tag{17}$$

with

$$\widetilde{\Delta}_{ij} \equiv \frac{POT \cdot T \cdot \int_j \int F\left(E_\nu\right) \cdot \frac{d\sigma(E_\nu, K_{true\ j})}{dK_{true\ j}} \cdot D\left(E_\nu, K_{true\ j} K_{rec\ i}\right) \cdot \epsilon(E_\nu, K_{true\ j}, K_{rec\ i}) \cdot dE_\nu \cdot dK_{true\ j}}{POT \cdot T \cdot \int_j \int \overline{F}\left(E_\nu\right) \cdot \frac{d\sigma(E_\nu, K_{true\ j})}{dK_{true\ j}} \cdot dE_\nu \cdot dK_{true\ j}} \tag{18}$$

being the main smearing matrix that can be directly extracted from the Monte Carlo simulation:

$$\widetilde{\Delta}_{ij} = \frac{\text{(Selected no. of events in reco. K bin i from true K bin j after event weights)}}{\text{(Generated no. of events in true K bin j after event weights)}}, \tag{19}$$

which is also used to estimate the impact of various systematic uncertainties (e.g. neutrino flux, neutrino-argon interaction cross section, and detector systematics). Here $\overline{F}$ represents the nominal (or central value) of the $\nu_\mu$ neutrino flux. Furthermore,

$$\widetilde{F}_j \equiv POT \cdot T \cdot \int_j \int \overline{F}(E_\nu) \cdot dE_\nu \cdot dK_{true\ j} = POT \cdot T \cdot \left( \int \overline{F}(E_\nu) \cdot dE_\nu \right) \cdot \Delta K_{true\ j} \tag{20}$$

is a constant that can be calculated externally knowing the nominal $\nu_\mu$ neutrino flux and the $j$th bin width $\Delta K_{true\ j}$. Finally, the targeted signal to be unfolded is defined as:

$$S_j \equiv \frac{\int_j \int \overline{F}(E_\nu) \cdot \frac{d\sigma(E_\nu, K_{true\ j})}{dK_{true\ j}} \cdot dE_\nu \cdot dK_{true\ j}}{\int_j \int \overline{F}(E_\nu) \cdot dE_\nu \cdot dK_{true\ j}} = \frac{\langle d\sigma(E_\nu, K_{true\ j}) \rangle}{\langle dK_{true\ j} \rangle}, \tag{21}$$

is the (nominal) flux-averaged differential cross section of the true K bin $j$ that we pursue in the unfolding procedure. Mapping $R_{ij} = \widetilde{\Delta}_{ij} \cdot \widetilde{F}_j$ to Eq. (16), we have

$$M_i - B_i = \sum_j R_{ij} \cdot S_j, \tag{22}$$

which is essentially the master equation in Eq. (6).

## VII. ENERGY SMEARING MATRICES

Figure 25, 26 and 27 shows the smearing matrices for the reconstructed neutrino energy, muon energy and (visible) hadronic energy, respectively.

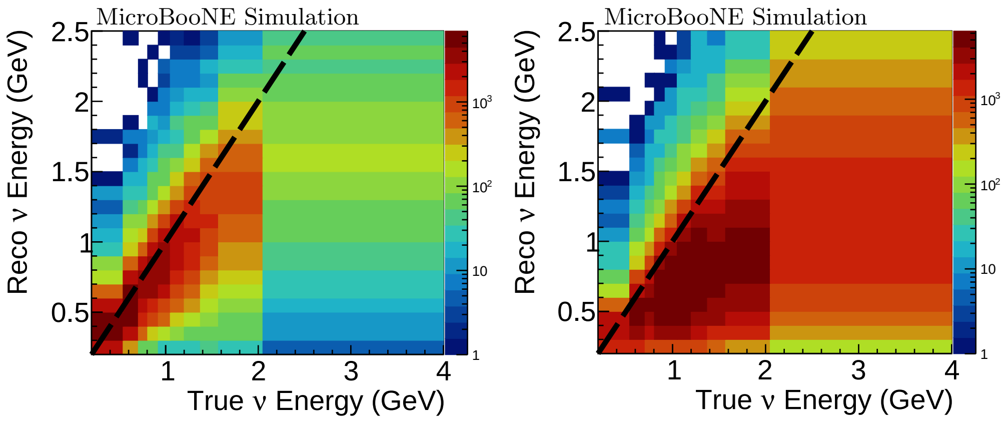


FIG. 25. Smearing matrix of the reconstructed neutrino energy for the selected $\nu_\mu$CC candidates: (left) FC events, (right) PC events.

## VIII. CROSS-SECTION RESULTS

The extracted $\nu_\mu$CC inclusive scattering cross section per nucleon as a function of neutrino energy, as well as the bin range and the flux-weighted bin center, is provided in the attached text file `microboone_cc_inclusive_cross_section.txt` and in Tab. III. Also provided in the same file are the measured $\nu_\mu$CC differential cross section per nucleon in muon energy $d\sigma/dE_\mu$ (Tab. IV) and the measured $\nu_\mu$CC differential cross section per nucleon in energy transfer $d\sigma/d\nu$ (Tab. V). The nominal BNB flux is available in the supplemental material of Ref. [30].

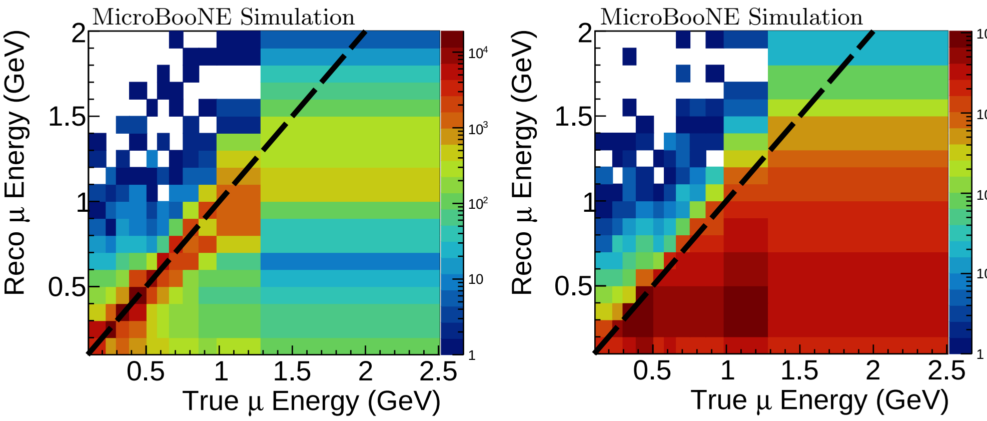


FIG. 26. Smearing matrix of the reconstructed muon energy for the selected $\nu_\mu$CC candidates: (left) FC events, (right) PC events.

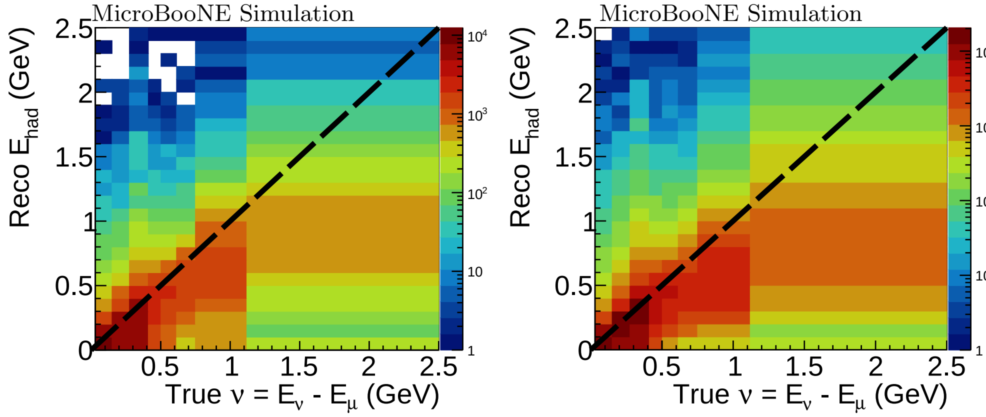


FIG. 27. Smearing matrix of the reconstructed hadronic (visible) energy for the selected $\nu_\mu$CC candidates: (left) FC events, (right) PC events.

| Bin Number | $E_\nu$ Range [GeV] | Flux-Weighted Bin Center [GeV] | $\sigma$ [$10^{-38}$ cm$^2$/nucleon] | Total Uncertainty [$10^{-38}$ cm$^2$/nucleon] |
|---|---|---|---|---|
| 1 | (0.2, 0.54] | 0.3818 | 0.3367 | 0.04369 |
| 2 | (0.54, 0.705] | 0.622 | 0.6751 | 0.06562 |
| 3 | (0.705, 0.805] | 0.7546 | 0.9309 | 0.08193 |
| 4 | (0.805, 0.92] | 0.8615 | 1.092 | 0.08613 |
| 5 | (0.92, 1.05] | 0.9833 | 1.192 | 0.09354 |
| 6 | (1.05, 1.2] | 1.122 | 1.234 | 0.1199 |
| 7 | (1.2, 1.375] | 1.282 | 1.292 | 0.1394 |
| 8 | (1.375, 1.57] | 1.463 | 1.401 | 0.1877 |
| 9 | (1.57, 2.05] | 1.735 | 1.571 | 0.2641 |
| 10 | (2.05, 4] | 2.619 | 1.977 | 0.378 |

TABLE III. $\nu_\mu$CC inclusive total cross section per nucleon in each neutrino energy bin with total statistical plus systematic uncertainty. The total uncertainty comes from the square root of the covariance matrix diagonal entries.

| Bin Number | $E_\mu$ Range [GeV] | Flux-Weighted Bin Center [GeV] | $d\sigma/dE_\mu$ [$10^{-38}$ cm$^2$/GeV/nucleon] | Total Uncertainty [$10^{-38}$ cm$^2$/GeV/nucleon] |
|---|---|---|---|---|
| 1 | (0.106, 0.226] | 0.1781 | 0.5278 | 0.07999 |
| 2 | (0.226, 0.296] | 0.2625 | 0.9569 | 0.08672 |
| 3 | (0.296, 0.386] | 0.3411 | 1.201 | 0.08685 |
| 4 | (0.386, 0.505] | 0.4446 | 1.127 | 0.0783 |
| 5 | (0.505, 0.577] | 0.5403 | 1.013 | 0.07523 |
| 6 | (0.577, 0.659] | 0.6174 | 0.8428 | 0.07323 |
| 7 | (0.659, 0.753] | 0.7051 | 0.7294 | 0.05955 |
| 8 | (0.753, 0.861] | 0.8052 | 0.6472 | 0.05695 |
| 9 | (0.861, 0.984] | 0.9194 | 0.5286 | 0.04919 |
| 10 | (0.984, 1.285] | 1.114 | 0.2798 | 0.0328 |
| 11 | (1.285, 2.506] | 1.6 | 0.04339 | 0.01233 |

TABLE IV. $\nu_\mu$CC inclusive differential cross section per nucleon in each muon energy bin with total statistical plus systematic uncertainty. The total uncertainty comes from the square root of the covariance matrix diagonal entries.

| Bin Number | $\nu$ Range [GeV] | Flux-Weighted Bin Center [GeV] | $d\sigma/d\nu$ [$10^{-38}$ cm$^2$/GeV/nucleon] | Total Uncertainty [$10^{-38}$ cm$^2$/GeV/nucleon] |
|---|---|---|---|---|
| 1 | (0.03, 0.15] | 0.1028 | 1.257 | 0.1282 |
| 2 | (0.15, 0.275] | 0.2129 | 1.355 | 0.1209 |
| 3 | (0.275, 0.411] | 0.3434 | 1.438 | 0.1103 |
| 4 | (0.411, 0.502] | 0.453 | 1.111 | 0.09028 |
| 5 | (0.502, 0.614] | 0.5539 | 0.7434 | 0.07889 |
| 6 | (0.614, 0.75] | 0.6776 | 0.4326 | 0.05177 |
| 7 | (0.75, 1.12] | 0.9064 | 0.1697 | 0.0316 |
| 8 | (1.12, 2.5] | 1.465 | 0.01551 | 0.01063 |

TABLE V. $\nu_\mu$CC inclusive differential cross section per nucleon in each energy transfer bin with total statistical plus systematic uncertainty. The total uncertainty comes from the square root of the covariance matrix diagonal entries.

To allow comparisons of these measurements with other model predictions, the covariance matrices of three cross-section measurements and the additional smearing matrices are provided in the attached text files: `microboone_cc_inclusive_cov_mat.txt` and `microboone_cc_inclusive_addtl_smr_mat.txt`, respectively. The covariance matrices are also shown in Fig. 28, consisting of both statistical and systematic uncertainties. The additional smearing is a result of the regularization in the data unfolding procedure, and should be applied to model predictions when comparing to our cross-section results. The code description below gives an example to properly re-smear the model prediction and calculate $\chi^2$:

```
/**
* Example C++/ROOT script for comparing the cross-section result
* with a model prediction
*
* v_ubdata: microboone unfolded cross section (vector)
* m_cov: covariance matrix
* v_model: model prediction of averaged cross section in each bin (vector)
* m_addtl_smr: additional smearing matrix
*/

int nbins = 11;
TMatrixD m_addtl_smr(nbins, nbins);
TMatrixD m_cov(nbins, nbins);
TVectorD v_ubdata(nbins);
TVectorD v_model(nbins);
```

```
for (int i=0; i<nbins; i++) {
  v_ubdata(i) = ...; // fill the MicroBooNE measurement
  v_model(i) = ...; // fill the model preidiction
  for (int j=0; j<nbins; j++) {
    m_addtl_smr(i,j) = ... // fill the smearing matrix
                           // e.g., m_addtl_smr(0,1) is row 0, column 1
    m_cov(i,j) = ... // fill the covariance matrix
  }
}
// re-smeared model prediction
TVectorD v_model_smr = m_addtl_smr * v_model;

// convert vector to matrix for computation
TMatrixD m_model_smr(1,nbins), m_ubdata(1,nbins);
for(int i=0; i<nbins; i++) {
  m_model_smr(0,i)=v_model_smr(i);
  m_ubdata(0,i)=v_ubdata(i);
}

// calculate chi2
TMatrixD m = m_model_smr - m_ubdata;
TMatrixD mT = m_model_smr - m_ubdata;
mT.T();
m_cov.Invert();
auto mret = m * m_cov * mT;
printf("chi2/dof=%.1f/%d\n", mret(0,0), nbins);
```

## IX. 1-BIN TOTAL CROSS SECTION (200-4000 MEV)

We also extracted the flux-integrated total cross section by following the same Wiener-SVD unfolding procedure except that we begin with 25 reconstructed energy bins for both FC and PC and end up with 1 true-energy bin from 200 MeV to 4000 MeV. The result is $(0.932 \pm 0.065) \times 10^{-38}$ cm$^2$/nucleon. For this flux-integrated total cross section, we provide the breakdown of uncertainties relative to the MC in Tab. VI, which is about 10% lower than the measurement from real data. One should note that the neutrino energy range for this measurement is narrower than the range in Ref. [30], resulting in a smaller flux uncertainty.

| Source of uncertainty | Relative uncertainty to MC truth |
|---|---|
| Data statistics | 0.97% |
| MC statistics (MC + EXT) | 0.31% |
| Xs systematics (Signal + Background) | 1.50% |
| Xs systematics (Signal only) | 1.11% |
| Xs systematics (Background only) | 1.19% |
| Flux systematics | 6.94% |
| Detector systematics | 1.34% |
| Additional DIRT | 0.053% |
| POT uncertainties | 2% |
| Target Nuclei | 1% |
| Total | 7.61% |

TABLE VI. Summary of uncertainties for the flux-integrated (200 MeV to 4 GeV) total cross section (Xs). The relative uncertainties are provided with relative to the MC truth total cross section, which is about 10% lower than the actual measurement from the real data.

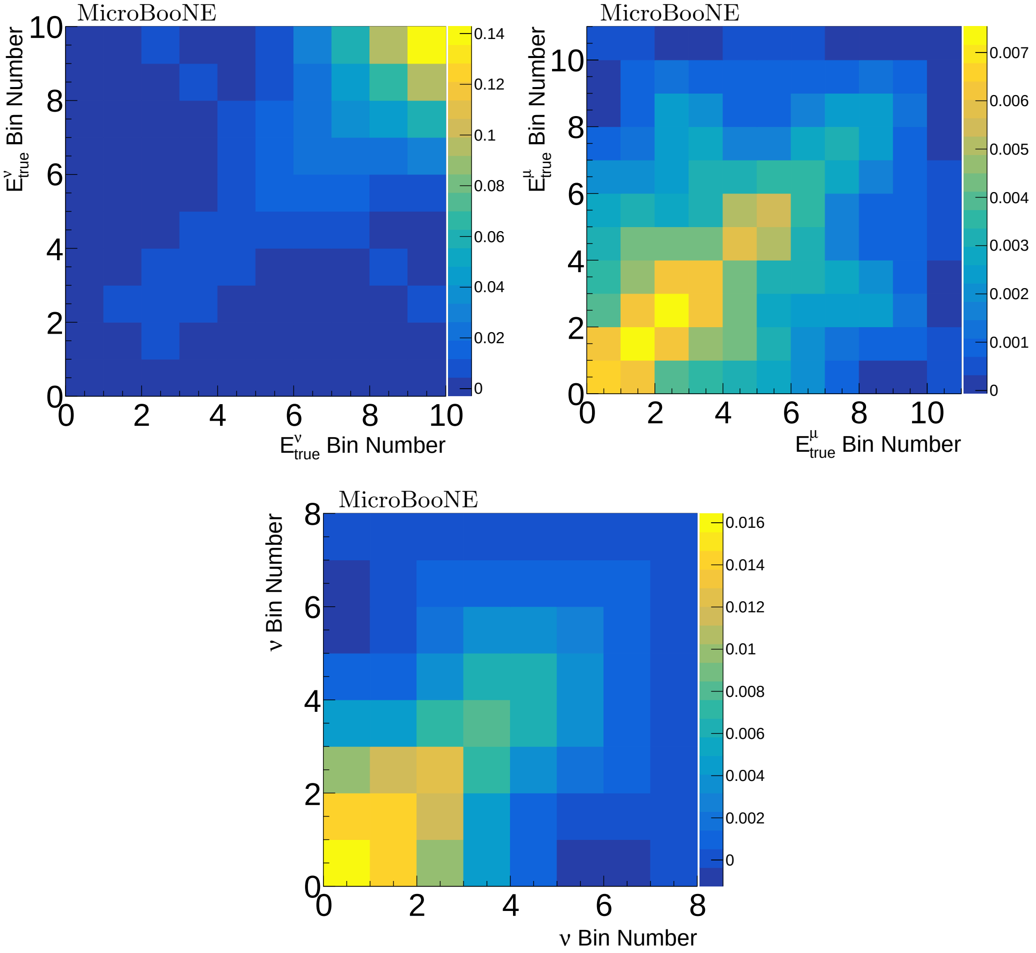


FIG. 28. Total covariance matrices in different energy bins for (a) total cross section per nucleon as a function of neutrino energy, (b) differential cross section per nucleon as a function of muon energy, and (c) differential cross section per nucleon as a function of energy transfer.


[1] Steve Baker and Robert D. Cousins. Clarification of the Use of Chi Square and Likelihood Functions in Fits to Histograms. *Nucl. Instrum. Meth.*, 221:437–442, 1984.

[2] Xiangpan Ji, Wenqiang Gu, Xin Qian, Hanyu Wei, and Chao Zhang. Combined Neyman–Pearson chi-square: An improved approximation to the Poisson-likelihood chi-square. *Nucl. Instrum. Meth. A*, 961:163677, 2020, 1903.07185.

[3] Morris L Eaton. Multivariate statistics: a vector space approach. *John Wiley and Sons*, pages 116–117, 1983.

[4] R.C. Carrasco and E. Oset. Interaction of real photons with nuclei from 100 to 500 mev. *Nuclear Physics A*, 536(3):445–508, 1992.

[5] Jaroslaw A. Nowak. Four Momentum Transfer Discrepancy in the Charged Current $\pi^+$ Production in the MiniBooNE: Data vs. Theory. *AIP Conf. Proc.*, 1189(1):243–248, 2009, 0909.3659.

[6] Konstantin S. Kuzmin, Vladimir V. Lyubushkin, and Vadim A. Naumov. Lepton polarization in neutrino nucleon interactions. *Mod. Phys. Lett. A*, 19:2815–2829, 2004, hep-ph/0312107.

[7] Ch. Berger and L. M. Sehgal. Lepton mass effects in single pion production by neutrinos. *Phys. Rev. D*, 76:113004, Dec 2007.

[8] Krzysztof M. Graczyk and Jan T. Sobczyk. Erratum: Form factors in the quark resonance model [phys. rev. d 77, 053001 (2008)]. *Phys. Rev. D*, 79:079903, Apr 2009.

[9] Ch. Berger and L. M. Sehgal. Partially conserved axial vector current and coherent pion production by low energy neutrinos. *Phys. Rev. D*, 79:053003, Mar 2009.

[10] D. Ashery, I. Navon, G. Azuelos, H. K. Walter, H. J. Pfeiffer, and F. W. Schlepütz. True absorption and scattering of pions on nuclei. *Phys. Rev. C*, 23:2173–2185, May 1981.

[11] Ko Abe et al. Measurement of double-differential muon neutrino charged-current interactions on $C_8H_8$ without pions in the final state using the T2K off-axis beam. *Phys. Rev. D*, 93(11):112012, 2016, 1602.03652.

[12] C. Andreopoulos, A. Bell, D. Bhattacharya, F. Cavanna, J. Dobson, S. Dytman, H. Gallagher, P. Guzowski, R. Hatcher, P. Kehayias, A. Meregaglia, D. Naples, G. Pearce, A. Rubbia, M. Whalley, and T. Yang. The genie neutrino monte carlo generator. *Nuclear Instruments and Methods in Physics Research Section A: Accelerators, Spectrometers, Detectors and Associated Equipment*, 614(1):87–104, 2010.

[13] Costas Andreopoulos, Christopher Barry, Steve Dytman, Hugh Gallagher, Tomasz Golan, Robert Hatcher, Gabriel Perdue, and Julia Yarba. The GENIE Neutrino Monte Carlo Generator: Physics and User Manual. 10 2015, 1510.05494.

[14] C. H. Llewellyn Smith. Neutrino Reactions at Accelerator Energies. *Phys. Rept.*, 3:261–379, 1972.

[15] Teppei Katori. Meson Exchange Current (MEC) Models in Neutrino Interaction Generators. *AIP Conf. Proc.*, 1663(1):030001, 2015, 1304.6014.

[16] Dieter Rein and Lalit M Sehgal. Neutrino-excitation of baryon resonances and single pion production. *Annals of Physics*, 133(1):79–153, 1981.

[17] S G Mashnik, A J Sierk, K K Gudima, and M I Baznat. CEM03 and LAQGSM03—new modeling tools for nuclear applications. *Journal of Physics: Conference Series*, 41:340–351, may 2006.

[18] T. Golan, J. T. Sobczyk, and J. Zmuda. NuWro: the Wroclaw Monte Carlo Generator of Neutrino Interactions. *Nucl. Phys. B Proc. Suppl.*, 229-232:499–499, 2012.

[19] Jackie Schwehr, Dan Cherdack, and Rik Gran. GENIE implementation of IFIC Valencia model for QE-like 2p2h neutrino-nucleus cross section. 1 2016, 1601.02038.

[20] K. M. Graczyk, D. Kielczewska, P. Przewlocki, and J. T. Sobczyk. C(5)**A axial form factor from bubble chamber experiments. *Phys. Rev. D*, 80:093001, 2009, 0908.2175.

[21] Yoshinari Hayato. A neutrino interaction simulation program library NEUT. *Acta Phys. Polon. B*, 40:2477–2489, 2009.

[22] J. Nieves, F. Sanchez, I. Ruiz Simo, and M. J. Vicente Vacas. Neutrino Energy Reconstruction and the Shape of the CCQE-like Total Cross Section. *Phys. Rev. D*, 85:113008, 2012, 1204.5404.

[23] L. L. Salcedo, E. Oset, M. J. Vicente-Vacas, and C. Garcia-Recio. Computer Simulation of Inclusive Pion Nuclear Reactions. *Nucl. Phys. A*, 484:557–592, 1988.

[24] O. Buss, T. Gaitanos, K. Gallmeister, H. van Hees, M. Kaskulov, O. Lalakulich, A. B. Larionov, T. Leitner, J. Weil, and U. Mosel. Transport-theoretical Description of Nuclear Reactions. *Phys. Rept.*, 512:1–124, 2012, 1106.1344.

[25] Tina Leitner, L. Alvarez-Ruso, and U. Mosel. Charged current neutrino nucleus interactions at intermediate energies. *Phys. Rev. C*, 73:065502, 2006, nucl-th/0601103.

[26] Lothar Tiator and Sabit Kamalov. Maid analysis techniques. In *5th International Workshop on the Physics of Excited Nucleons*, 3 2006, nucl-th/0603012.

[27] Torbjorn Sjostrand, Stephen Mrenna, and Peter Z. Skands. PYTHIA 6.4 Physics and Manual. *JHEP*, 05:026, 2006, hep-ph/0603175.

[28] Júlia Tena-Vidal et al. Neutrino-Nucleon Cross-Section Model Tuning in GENIE v3. 4 2021, 2104.09179.

[29] Lukas Koch and Stephen Dolan. Treatment of flux shape uncertainties in unfolded, flux-averaged neutrino cross-section measurements. *Phys. Rev. D*, 102:113012, 2020, 2009.00552.

[30] P. Abratenko et al. First Measurement of Inclusive Muon Neutrino Charged Current Differential Cross Sections on Argon at $E_\nu \sim$0.8 GeV with the MicroBooNE Detector. *Phys. Rev. Lett.*, 123(13):131801, 2019, 1905.09694.
